# Supplementary material for: ControlVideo: Training-free Controllable Text-to-Video Generation
Source: arXiv:2305.13077 source file (2023-05-22)
Supplement: Supplementary file 1 [file supp_visualize.tex]

\begin{figure}[t]
%   \vspace{-1em}
  \begin{center}
  \includegraphics[width=.95\linewidth]{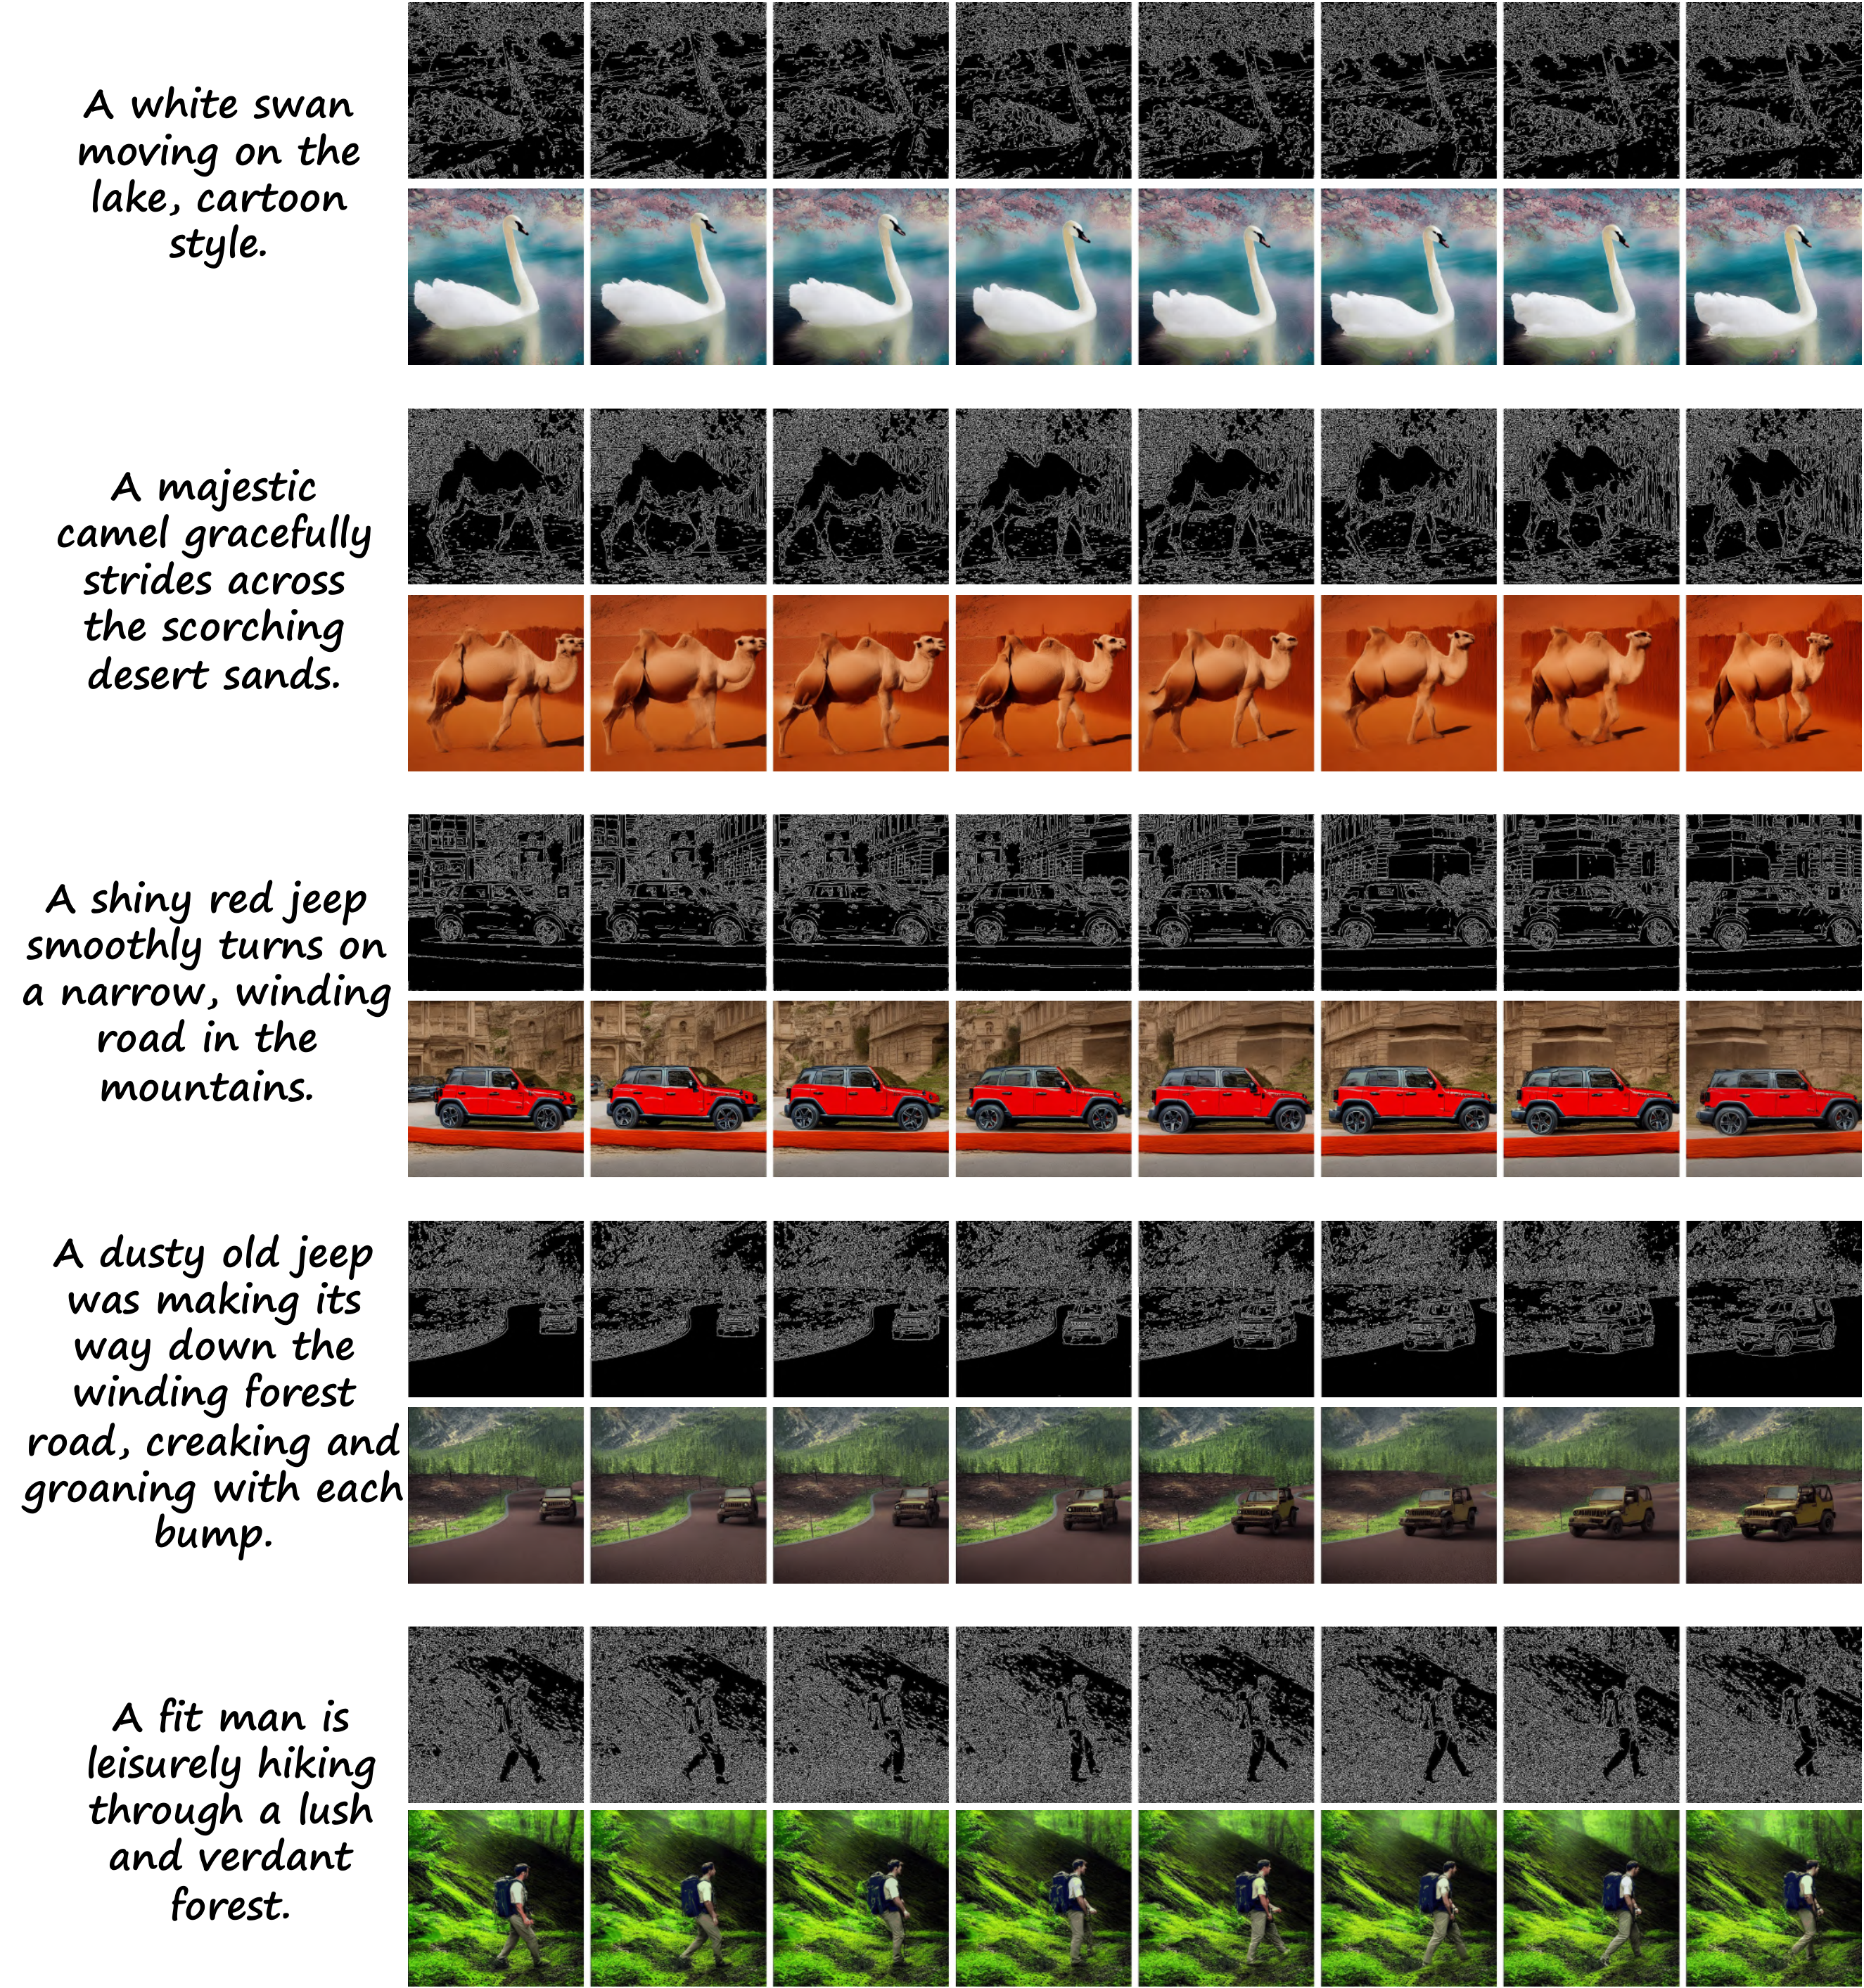}
  \end{center}
  \vspace{-1mm}
  \caption{
  \textbf{More video visualizations conditioned on canny edges.}
  \textbf{Results best seen at 500\% zoom.}
  }
    \label{fig:supp_canny}
  \vspace{-1mm}
\end{figure}

\begin{figure}[t]
%   \vspace{-1em}
  \begin{center}
  \includegraphics[width=.95\linewidth]{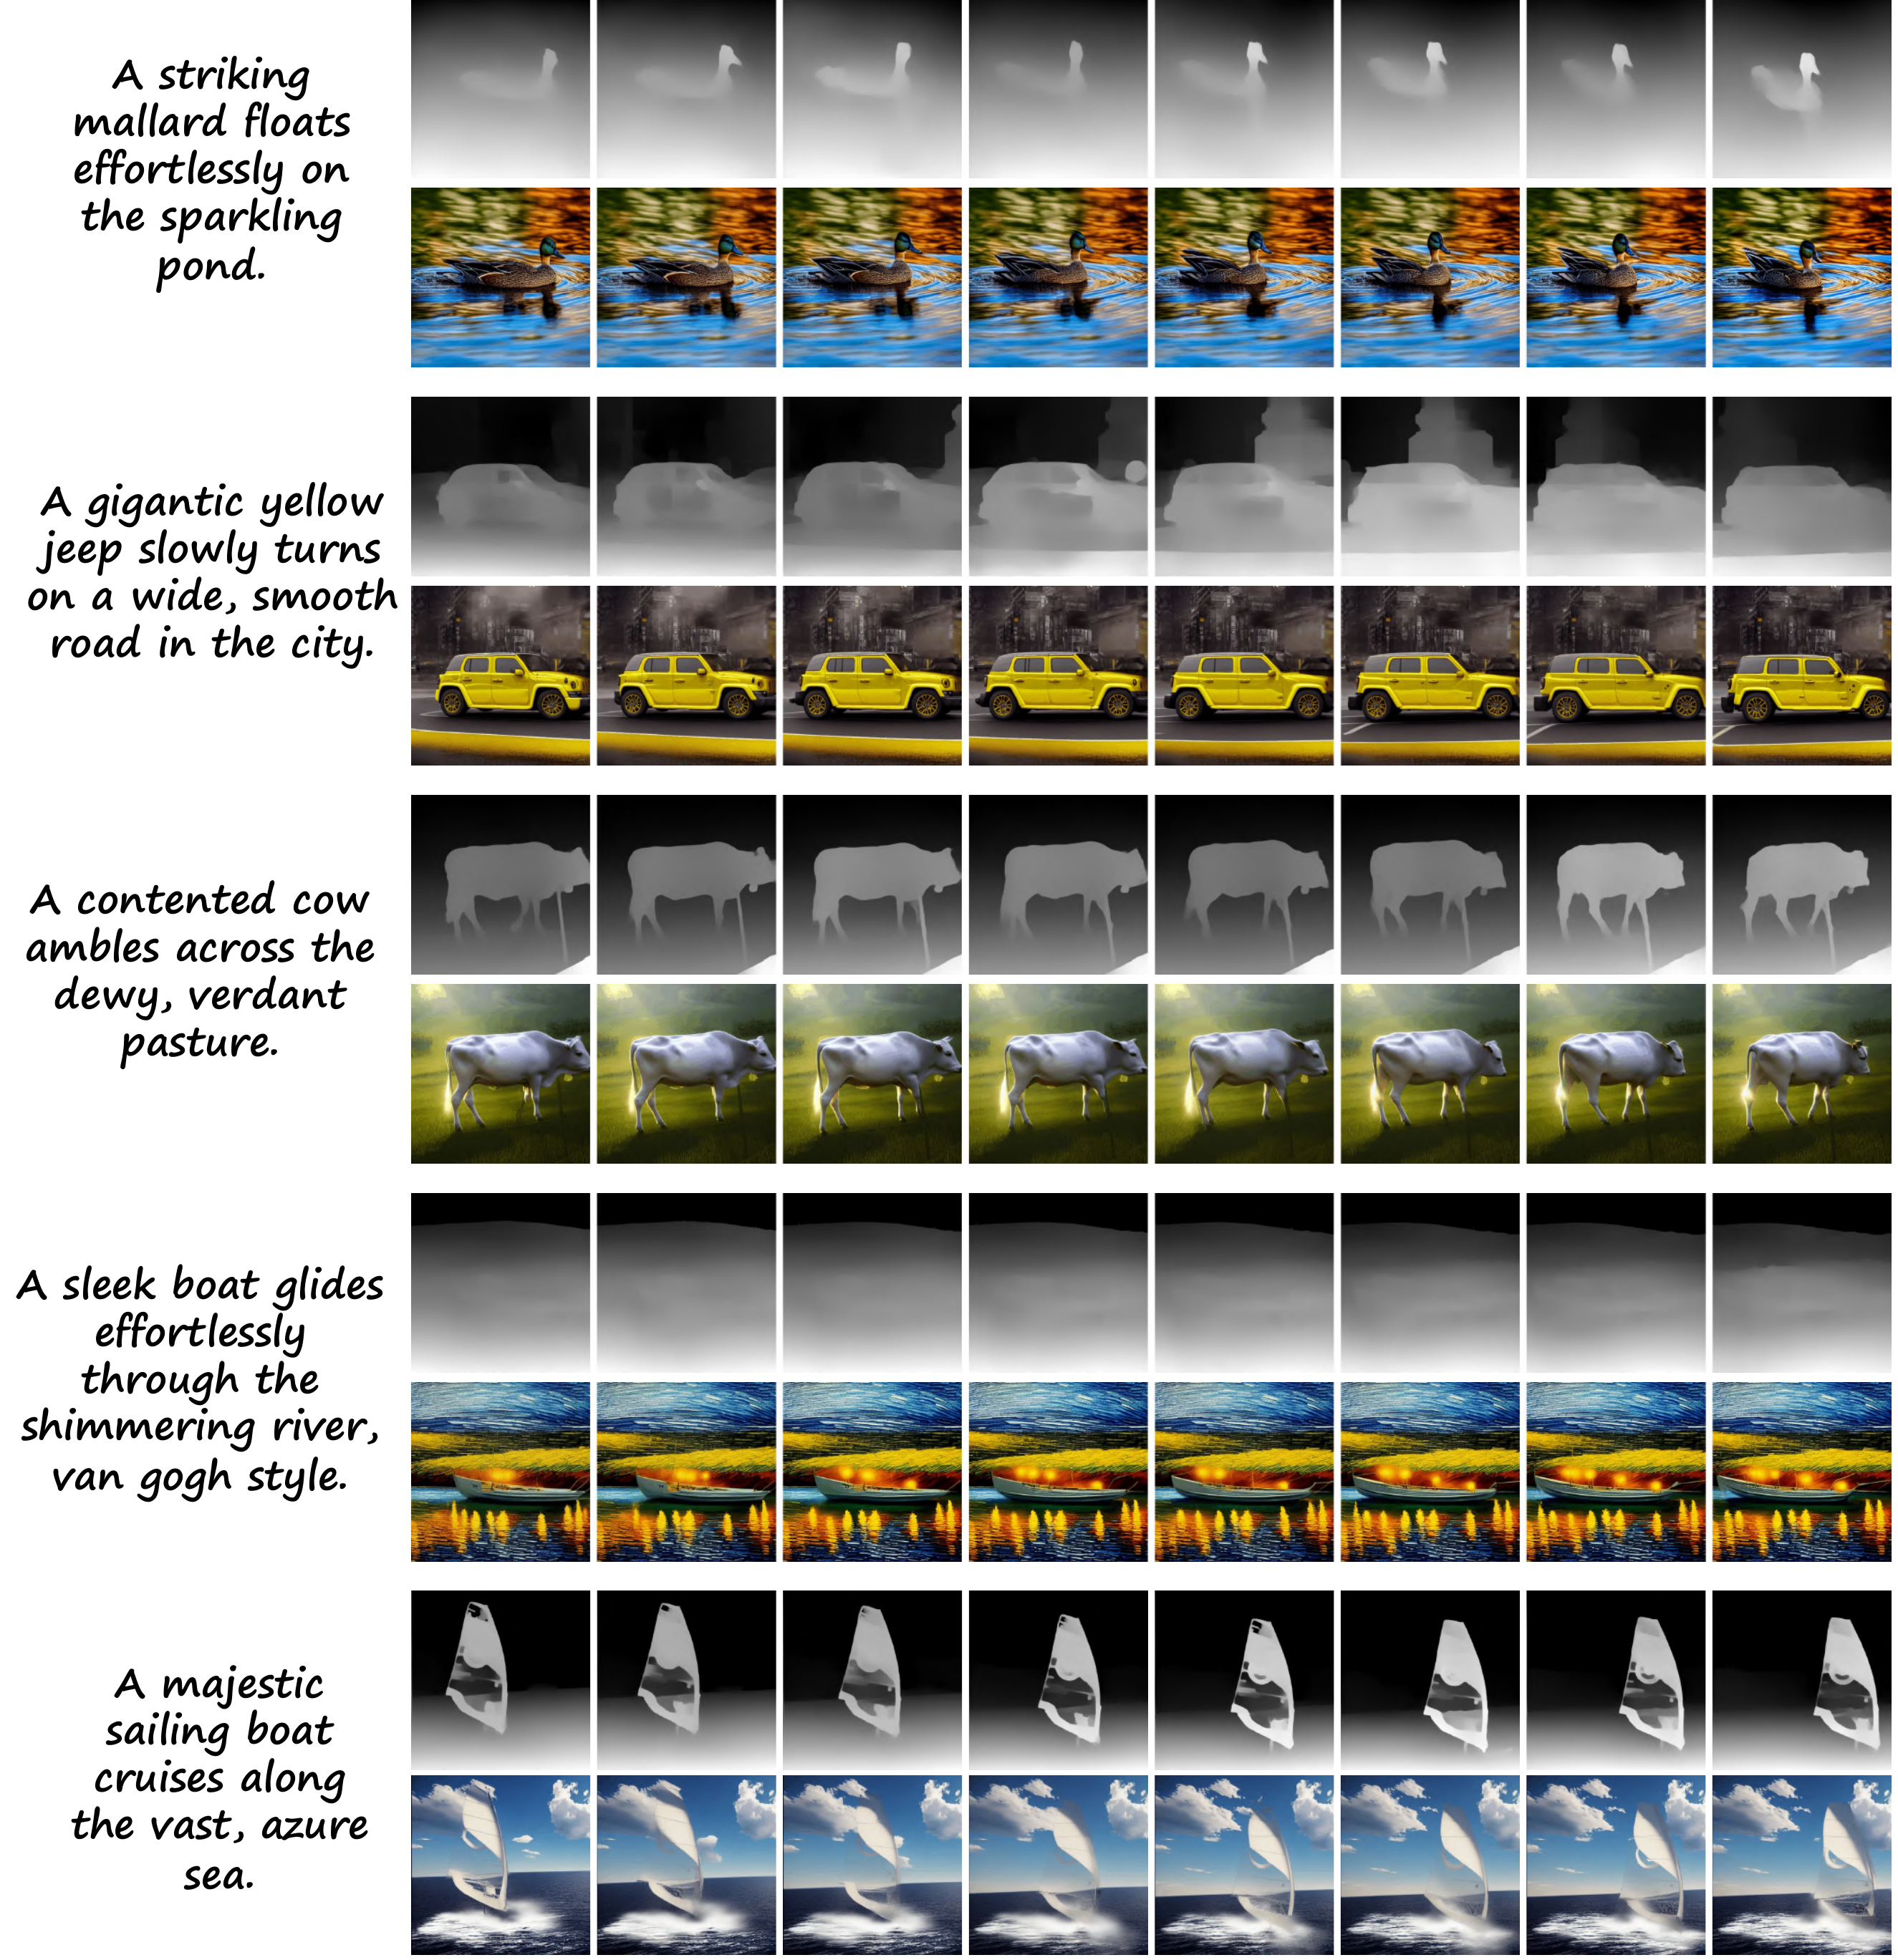}
  \end{center}
  \vspace{-1mm}
  \caption{
  \textbf{More video visualizations conditioned on depth maps.}
  \textbf{Results best seen at 500\% zoom.}
  }
    \label{fig:supp_depth}
  \vspace{-1mm}
\end{figure}

\begin{figure}[t]
%   \vspace{-1em}
  \begin{center}
  \includegraphics[width=.95\linewidth]{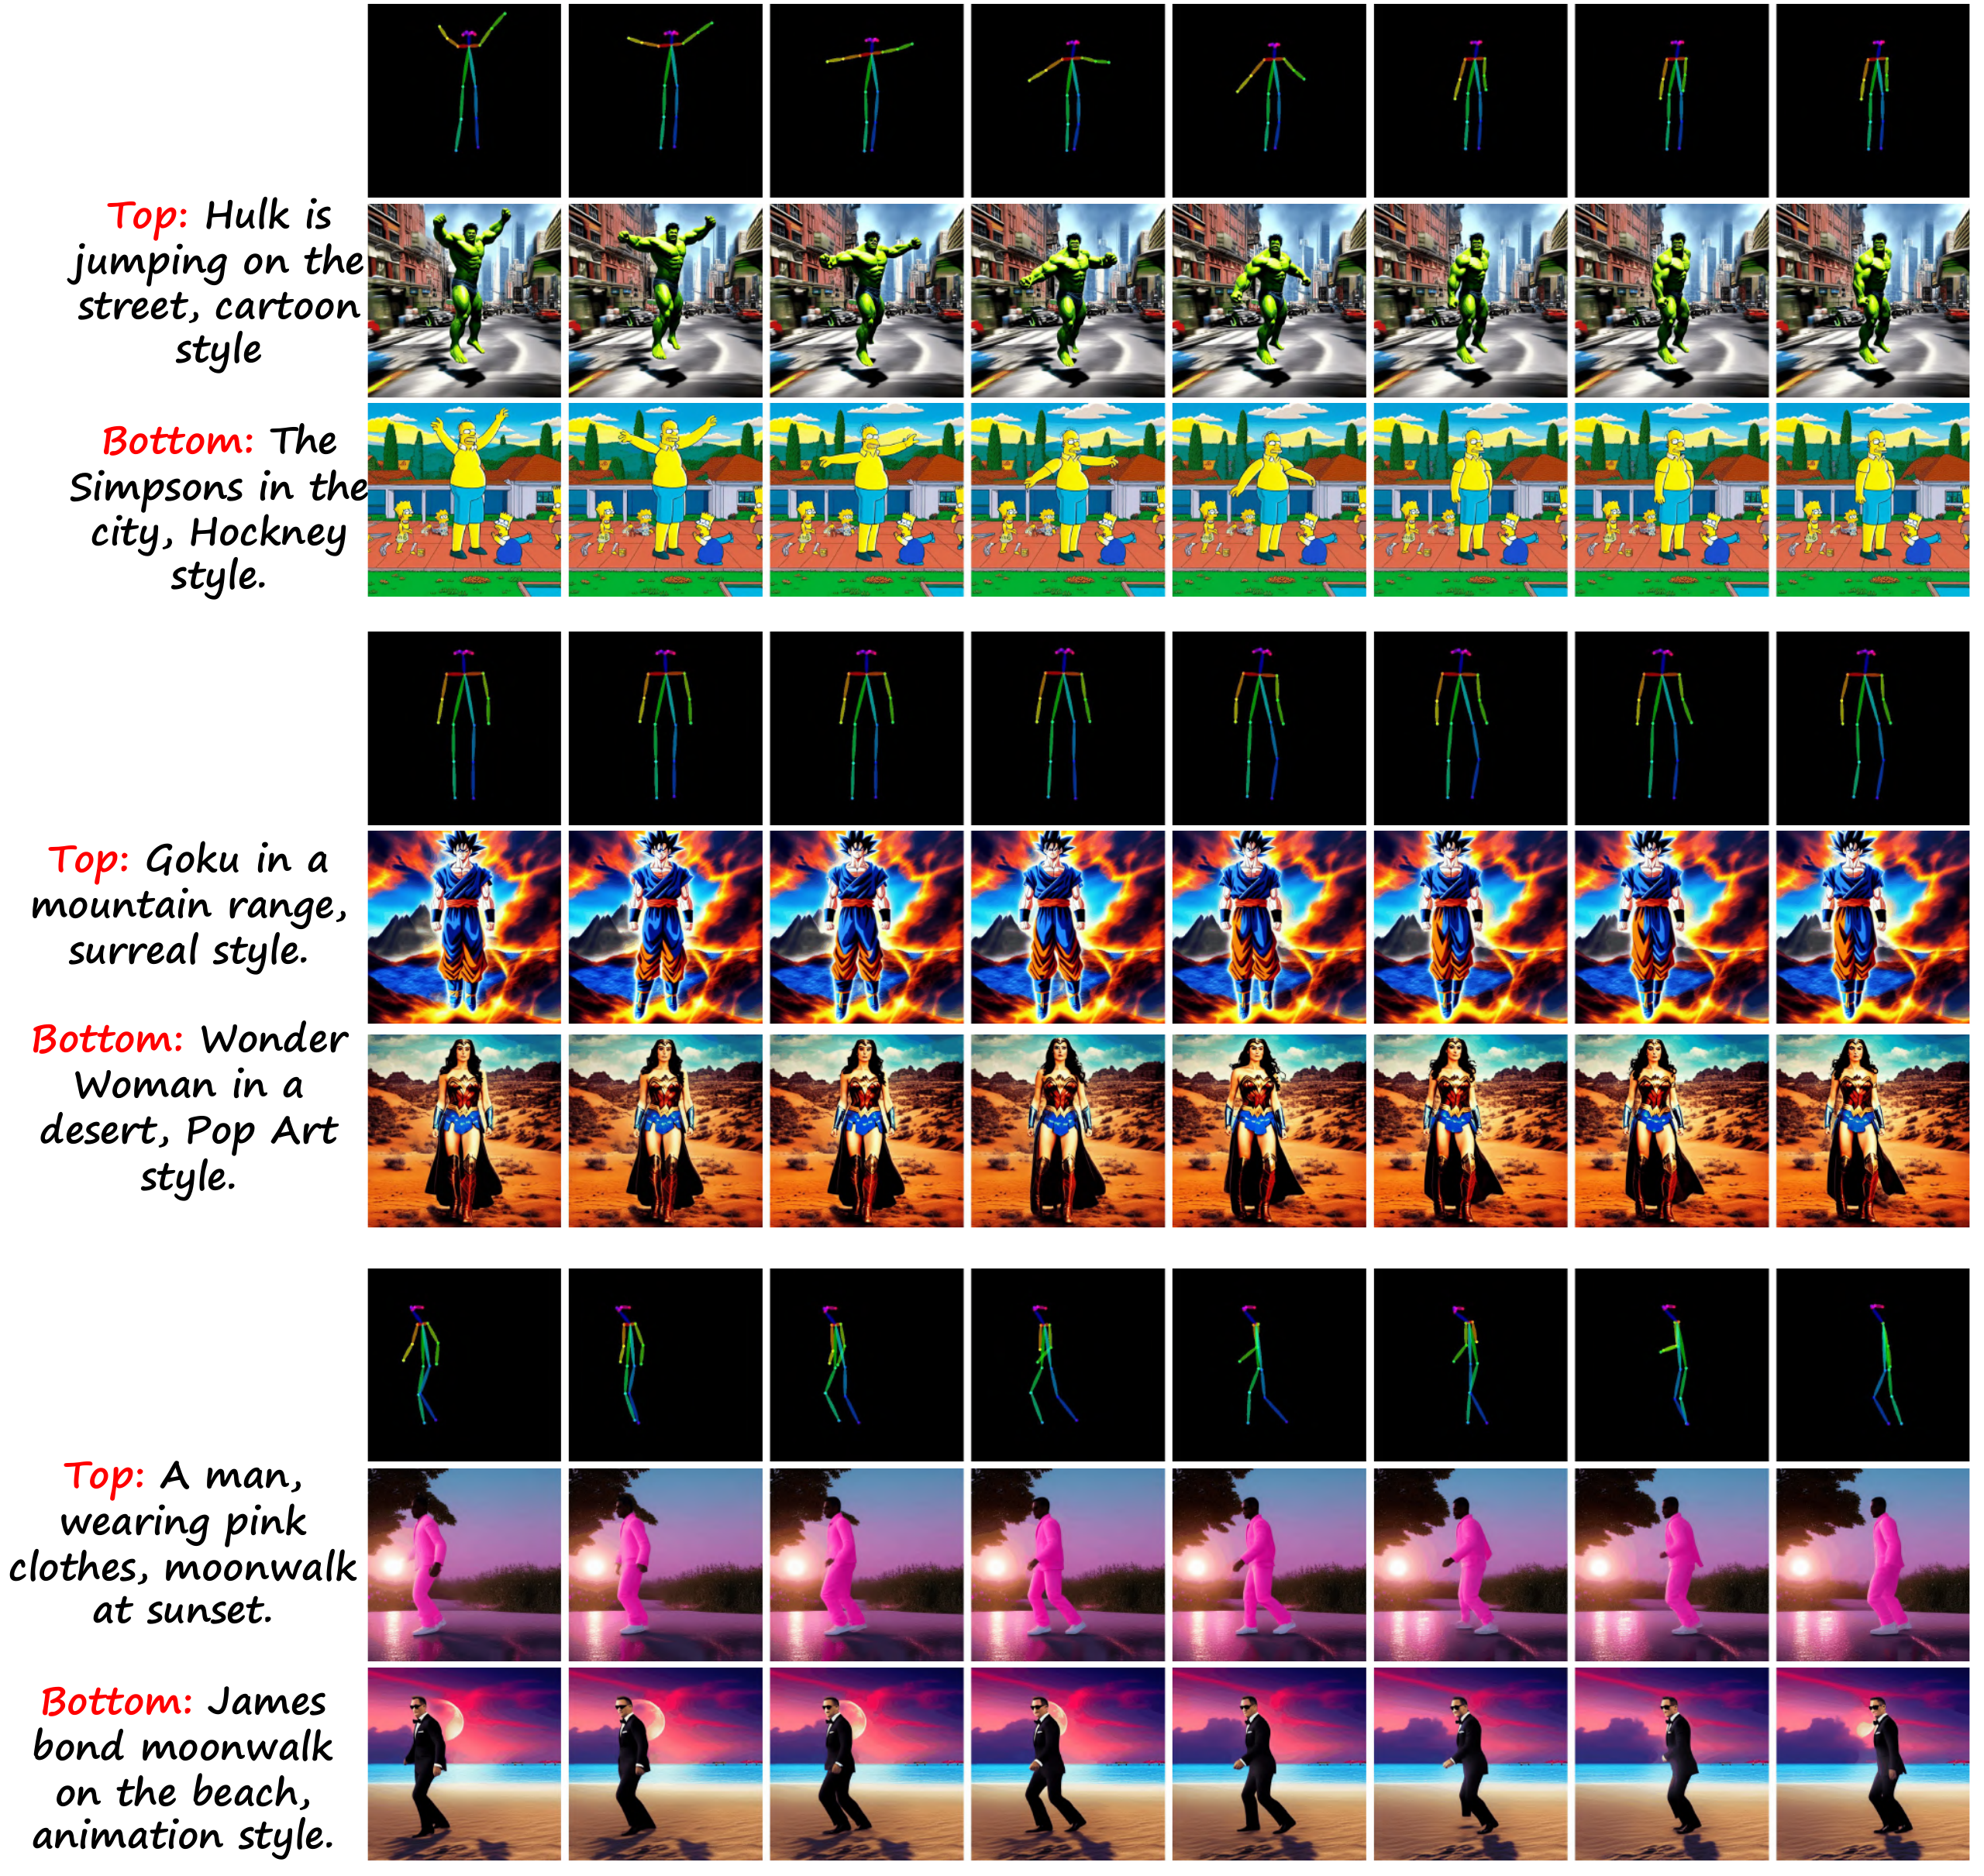}
  \end{center}
  \vspace{-1mm}
  \caption{
  \textbf{More video visualizations conditioned on human poses.}
  \textbf{Results best seen at 500\% zoom.}
  }
    \label{fig:supp_pose}
  \vspace{-1mm}
\end{figure}

\begin{figure}[t]
%   \vspace{-1em}
  \begin{center}
  \includegraphics[width=.9\linewidth]{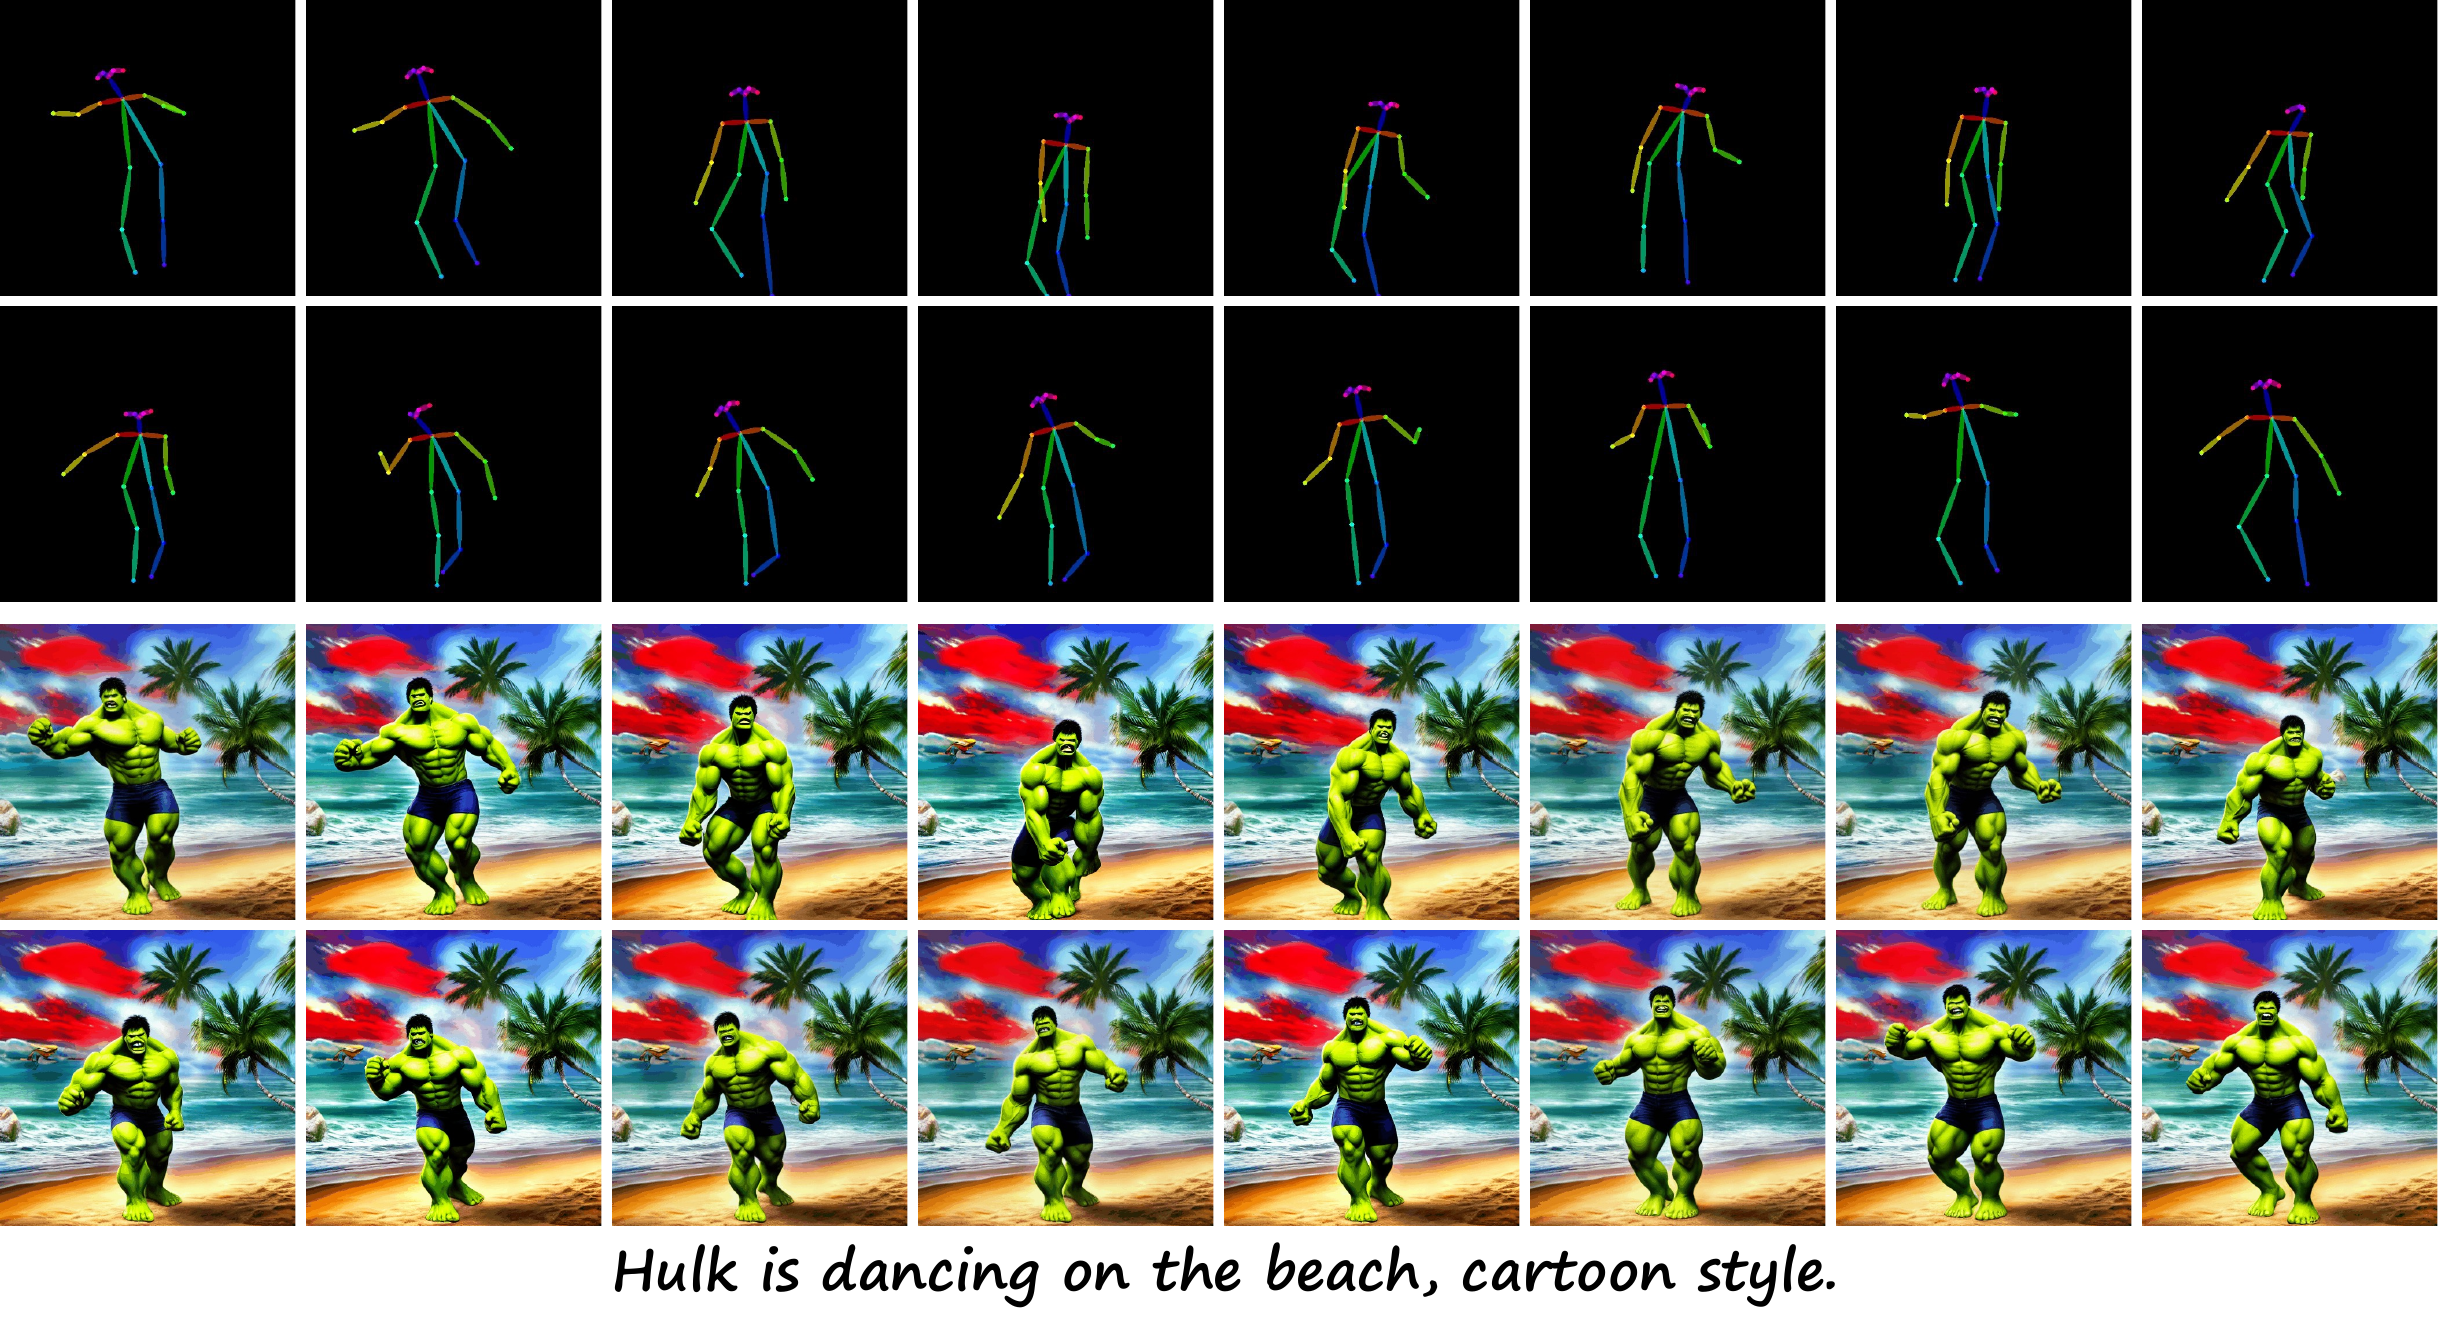}
  \end{center}
  \vspace{-1mm}
  \caption{
  \textbf{Additional long video visualization.}
  \textbf{Results best seen at 500\% zoom.}
  }
    \label{fig:supp_long}
  \vspace{-1mm}
\end{figure}

\begin{figure}[t]
%   \vspace{-1em}
  \begin{center}
  \includegraphics[width=.99\linewidth]{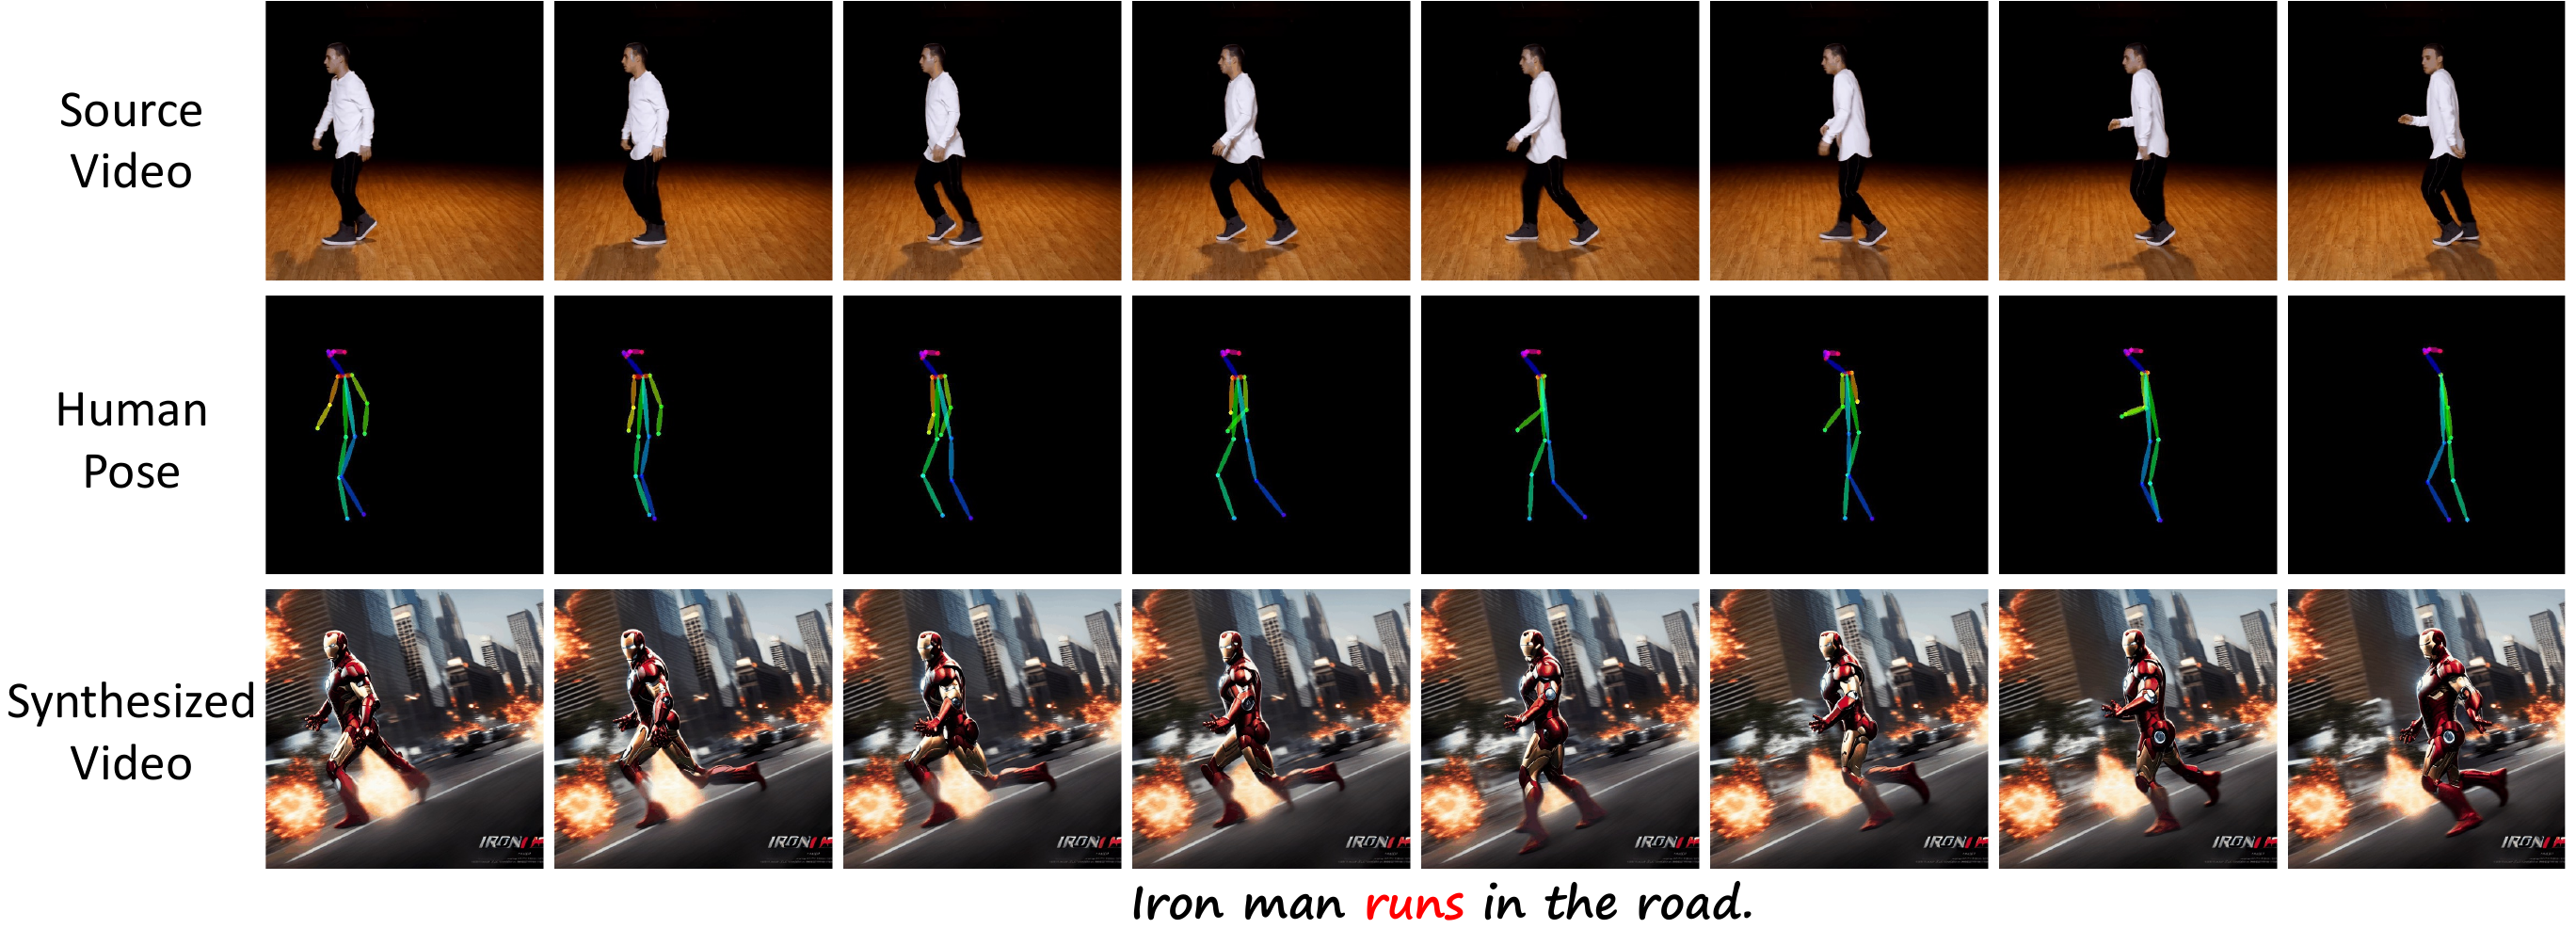}
  \end{center}
  \vspace{-1mm}
  \caption{\textbf{Limitation visualizations.}
  ControlVideo struggles with producing videos beyond input motion sequences.
  The motion of text prompt \texttt{Iron man \textcolor{red}{runs} on the street} does not align with the given sequential poses of \texttt{Michael Jackson's moonwalk}, which degrades the video quality and consistency.
  }
    \label{fig:supp_limitation}
  \vspace{-1mm}
\end{figure}
