# Supplementary material for: ControlVideo: Training-free Controllable Text-to-Video Generation
Source: arXiv:2305.13077 source file (2023-05-22)
Supplement: Supplementary file 2 [file supp_comare.tex]

\begin{figure}[t]
%   \vspace{-1em}
  \begin{center}
  \includegraphics[width=.99\linewidth]{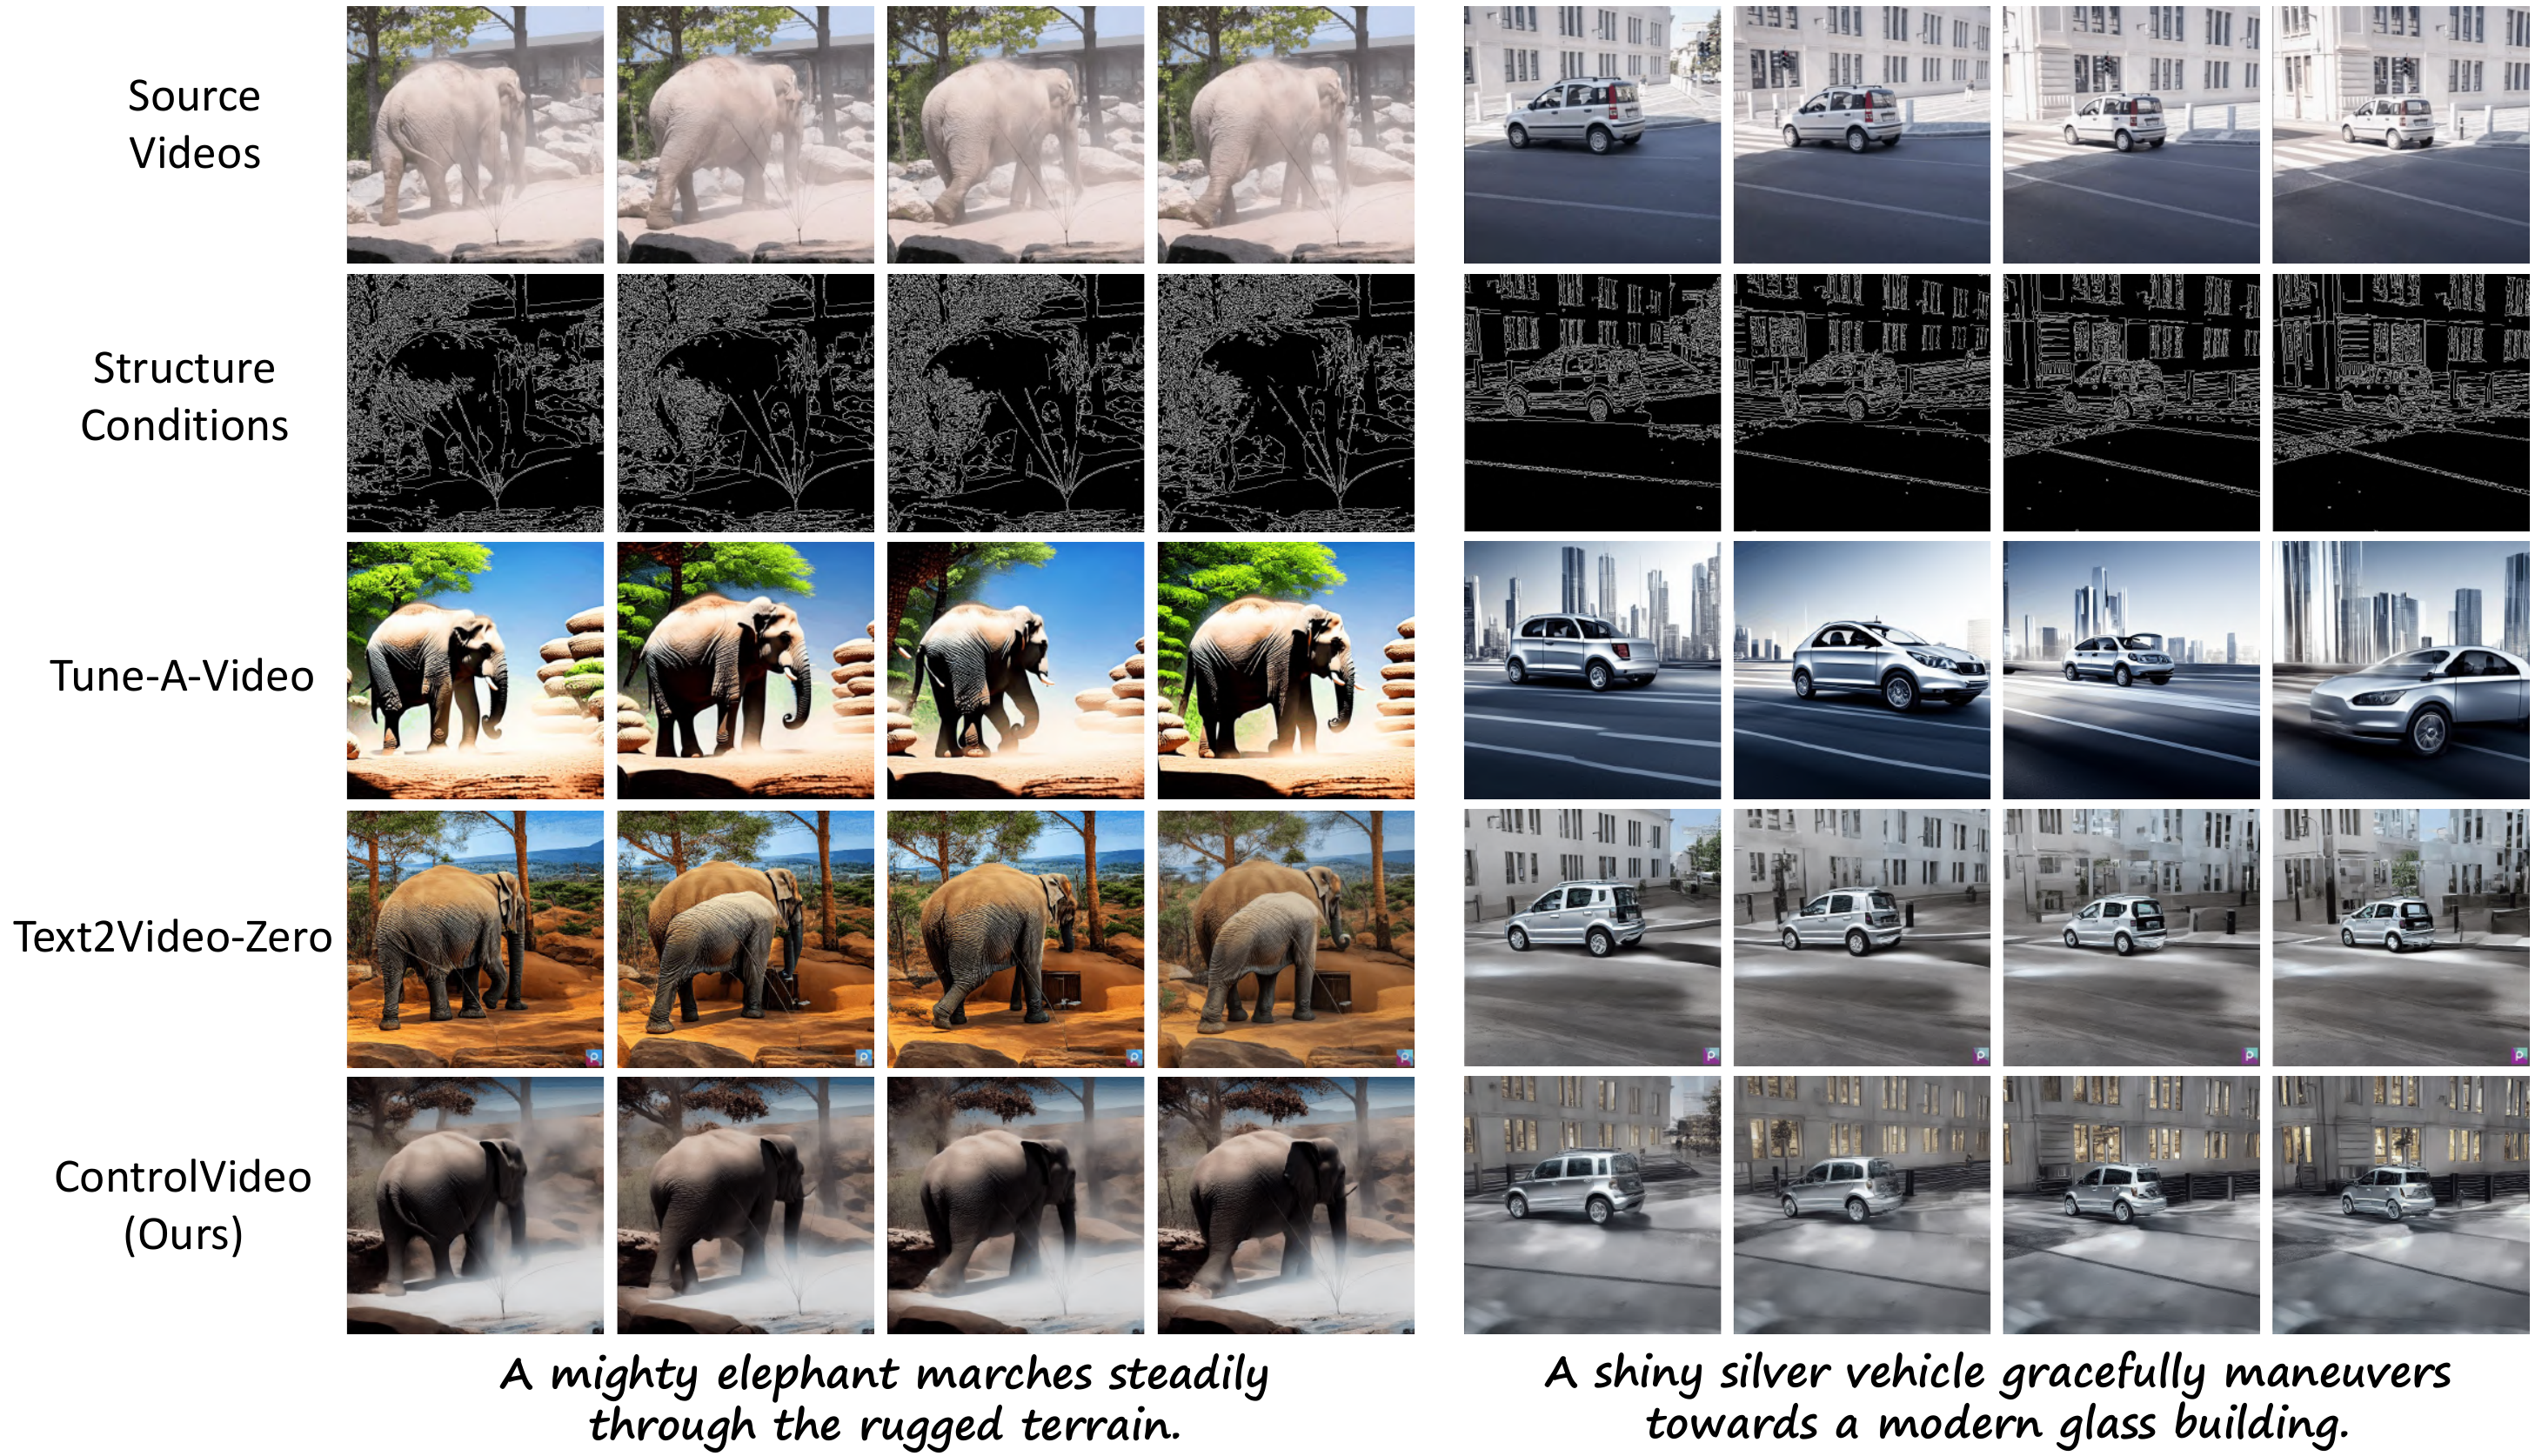}
  \end{center}
  \vspace{-1mm}
  \caption{
  \textbf{More qualitative comparisons conditioned on canny edges.}
  \textbf{Results best seen at 500\% zoom.}
  }
    \label{fig:supp_com_canny}
  \vspace{-1mm}
\end{figure}

\begin{figure}[t]
%   \vspace{-1em}
  \begin{center}
  \includegraphics[width=.99\linewidth]{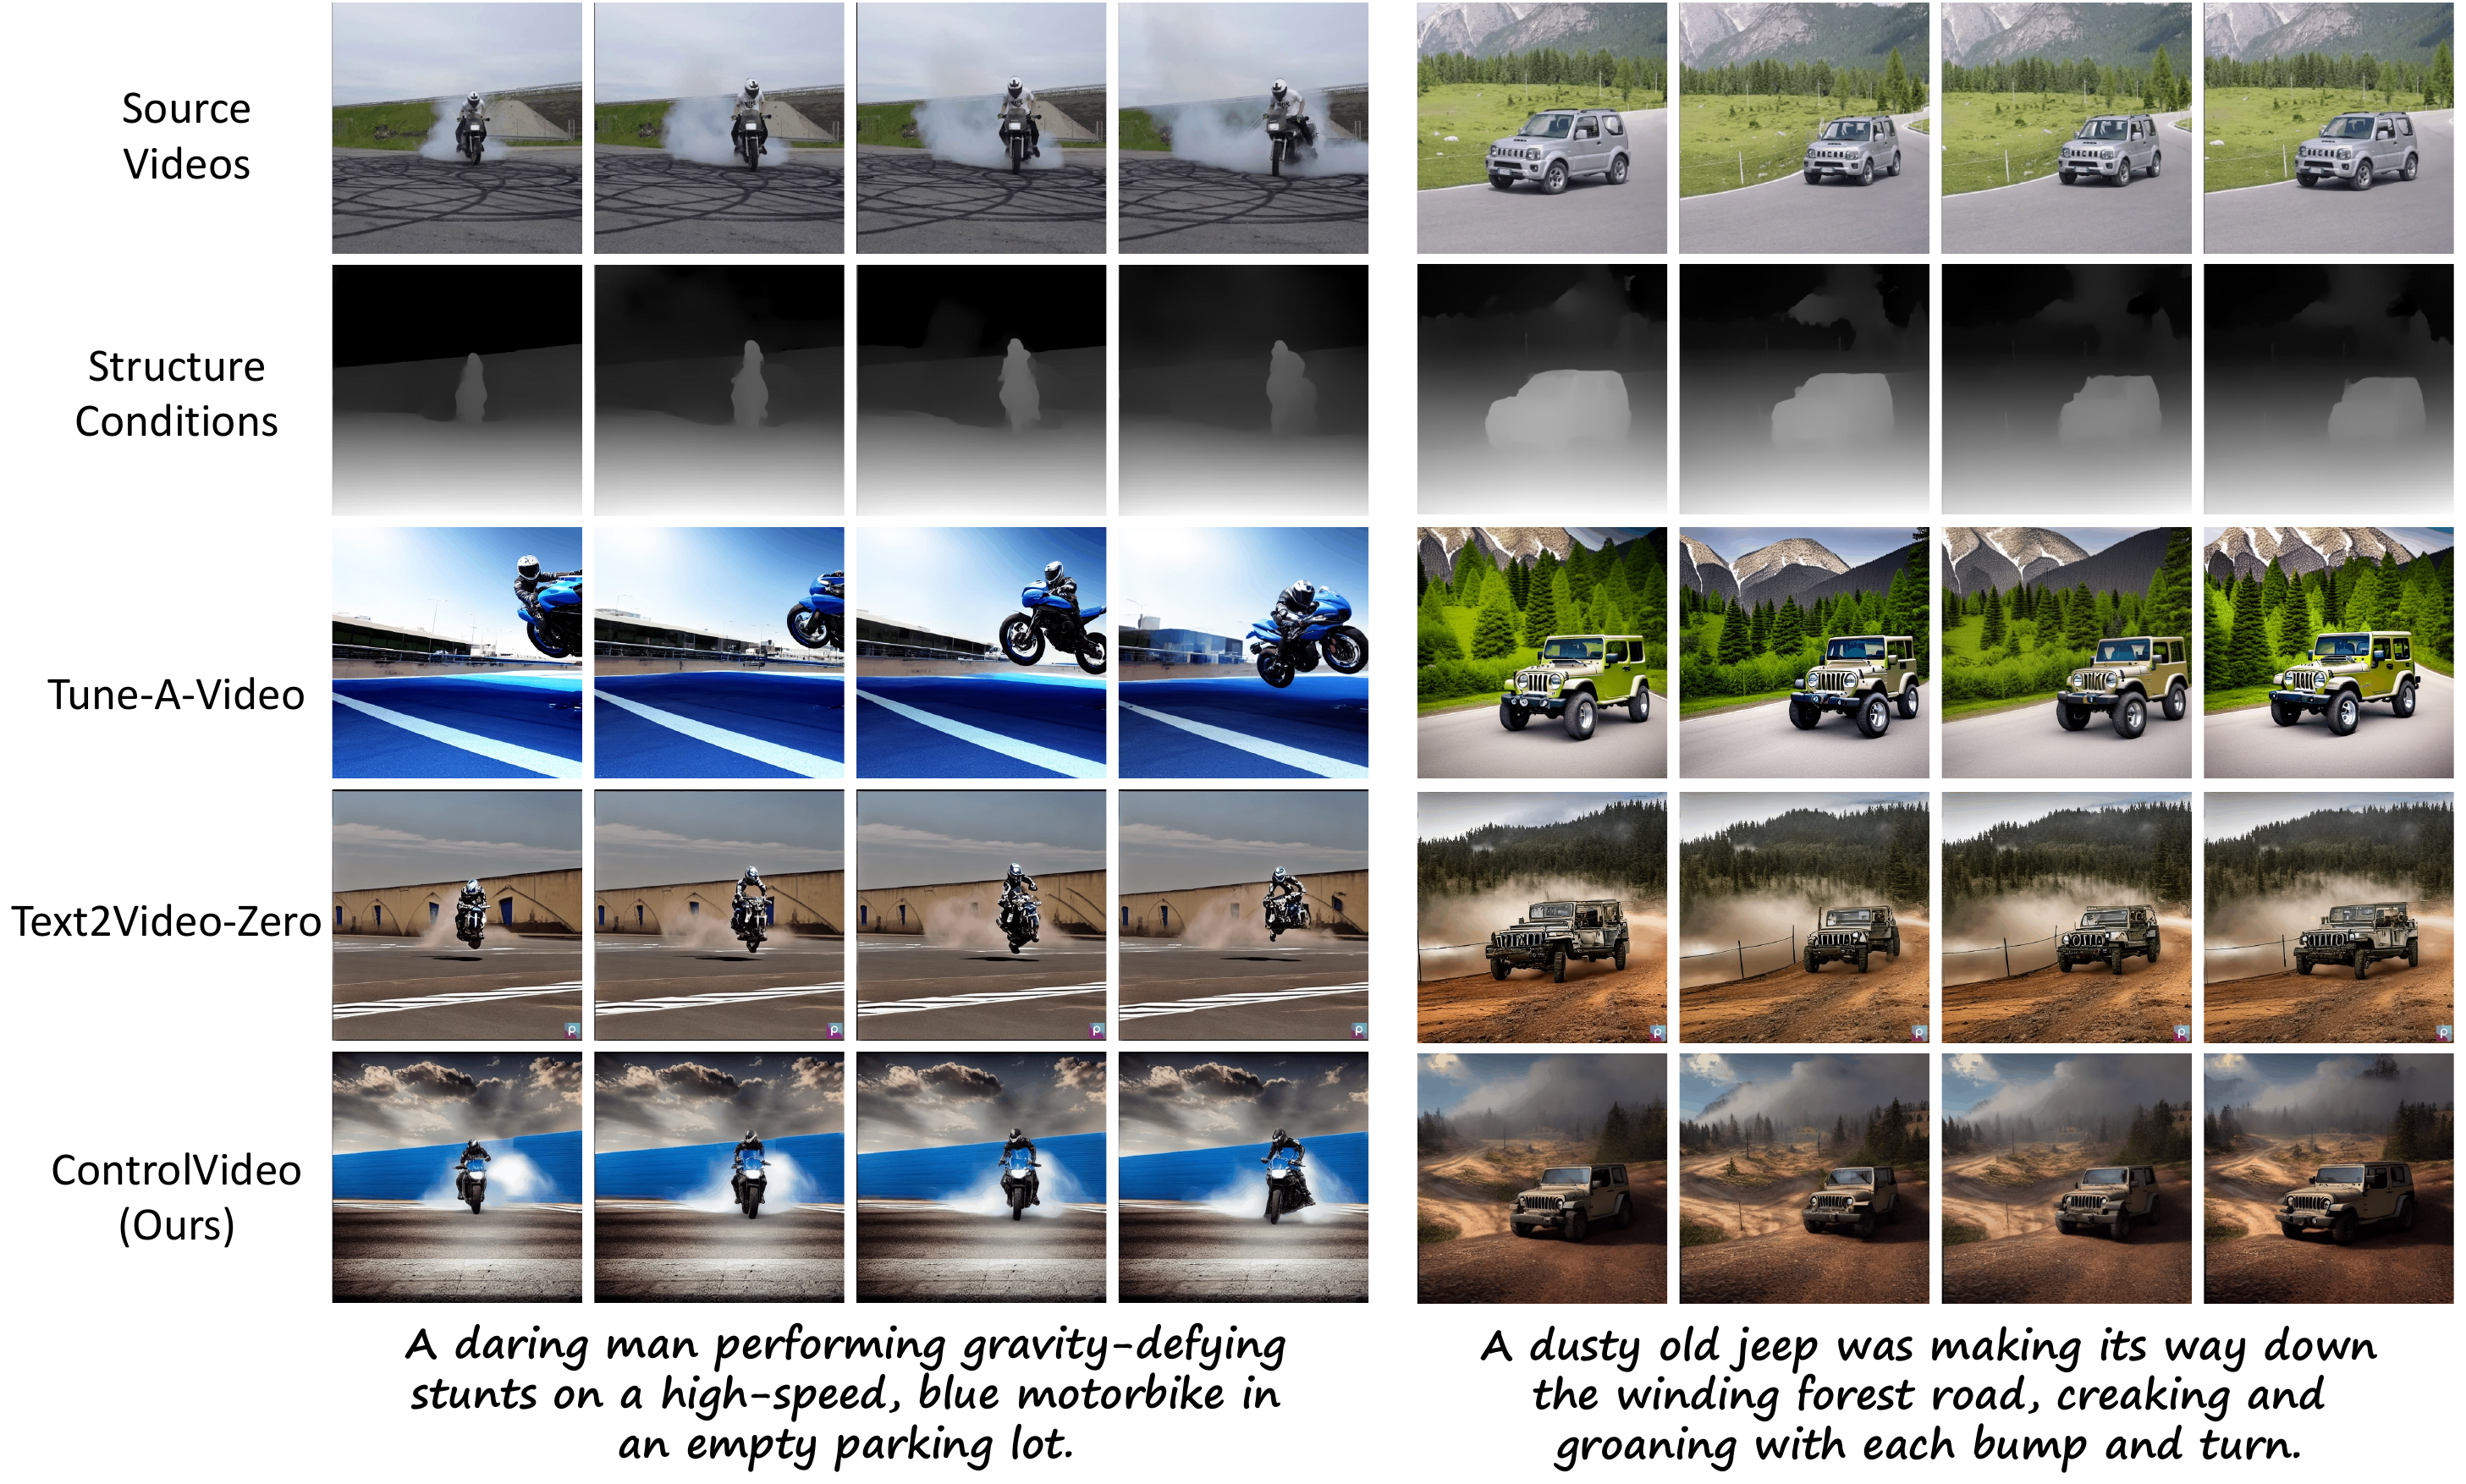}
  \end{center}
  \vspace{-1mm}
  \caption{
  \textbf{More qualitative comparisons conditioned on depth maps.}
  \textbf{Results best seen at 500\% zoom.}
  }
    \label{fig:supp_com_depth}
  \vspace{-1mm}
\end{figure}

\begin{figure}[t]
%   \vspace{-1em}
  \begin{center}
  \includegraphics[width=.99\linewidth]{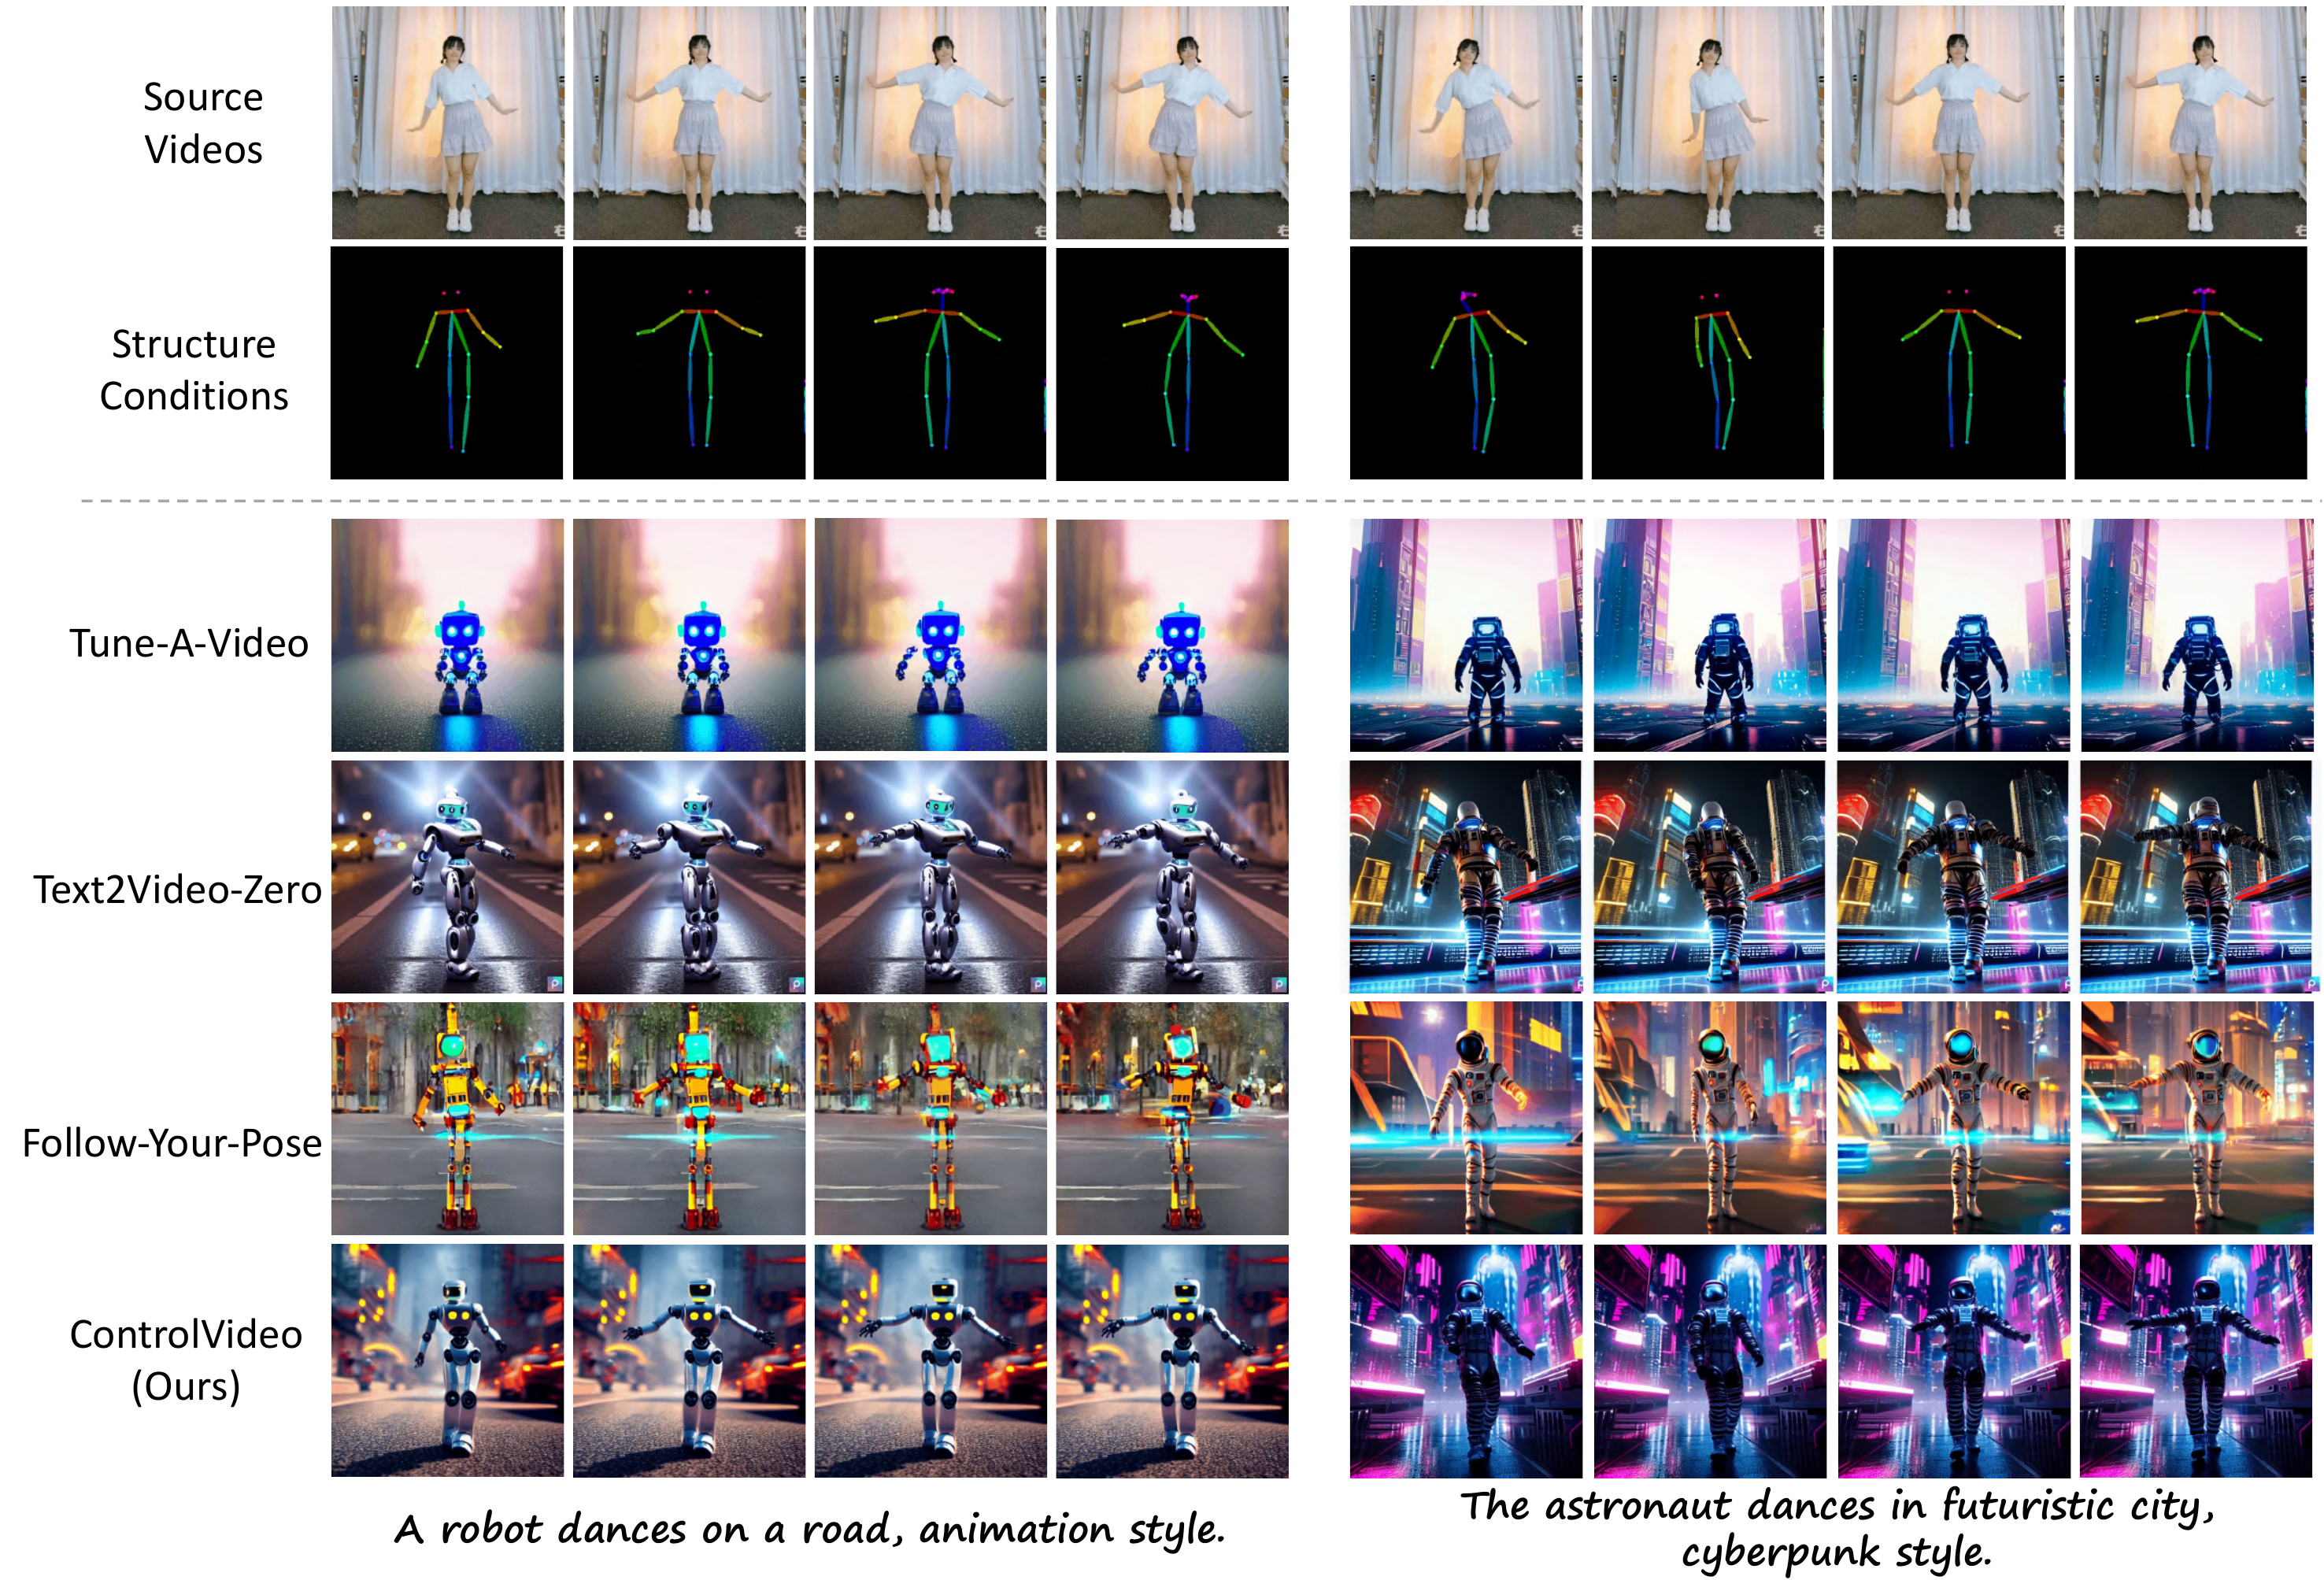}
  \end{center}
  \vspace{-1mm}
  \caption{
  \textbf{More qualitative comparisons conditioned on human poses.}
  \textbf{Results best seen at 500\% zoom.}
  }
    \label{fig:supp_com_pose}
  \vspace{-1mm}
\end{figure}
