# Supplementary material for: ControlVideo: Training-free Controllable Text-to-Video Generation
Source: arXiv:2305.13077 source file (2023-05-22)
Supplement: Supplementary file 3 [file supp_smoother.tex]

\begin{figure}[t]
%   \vspace{-1em}
  \begin{center}
  \includegraphics[width=.95\linewidth]{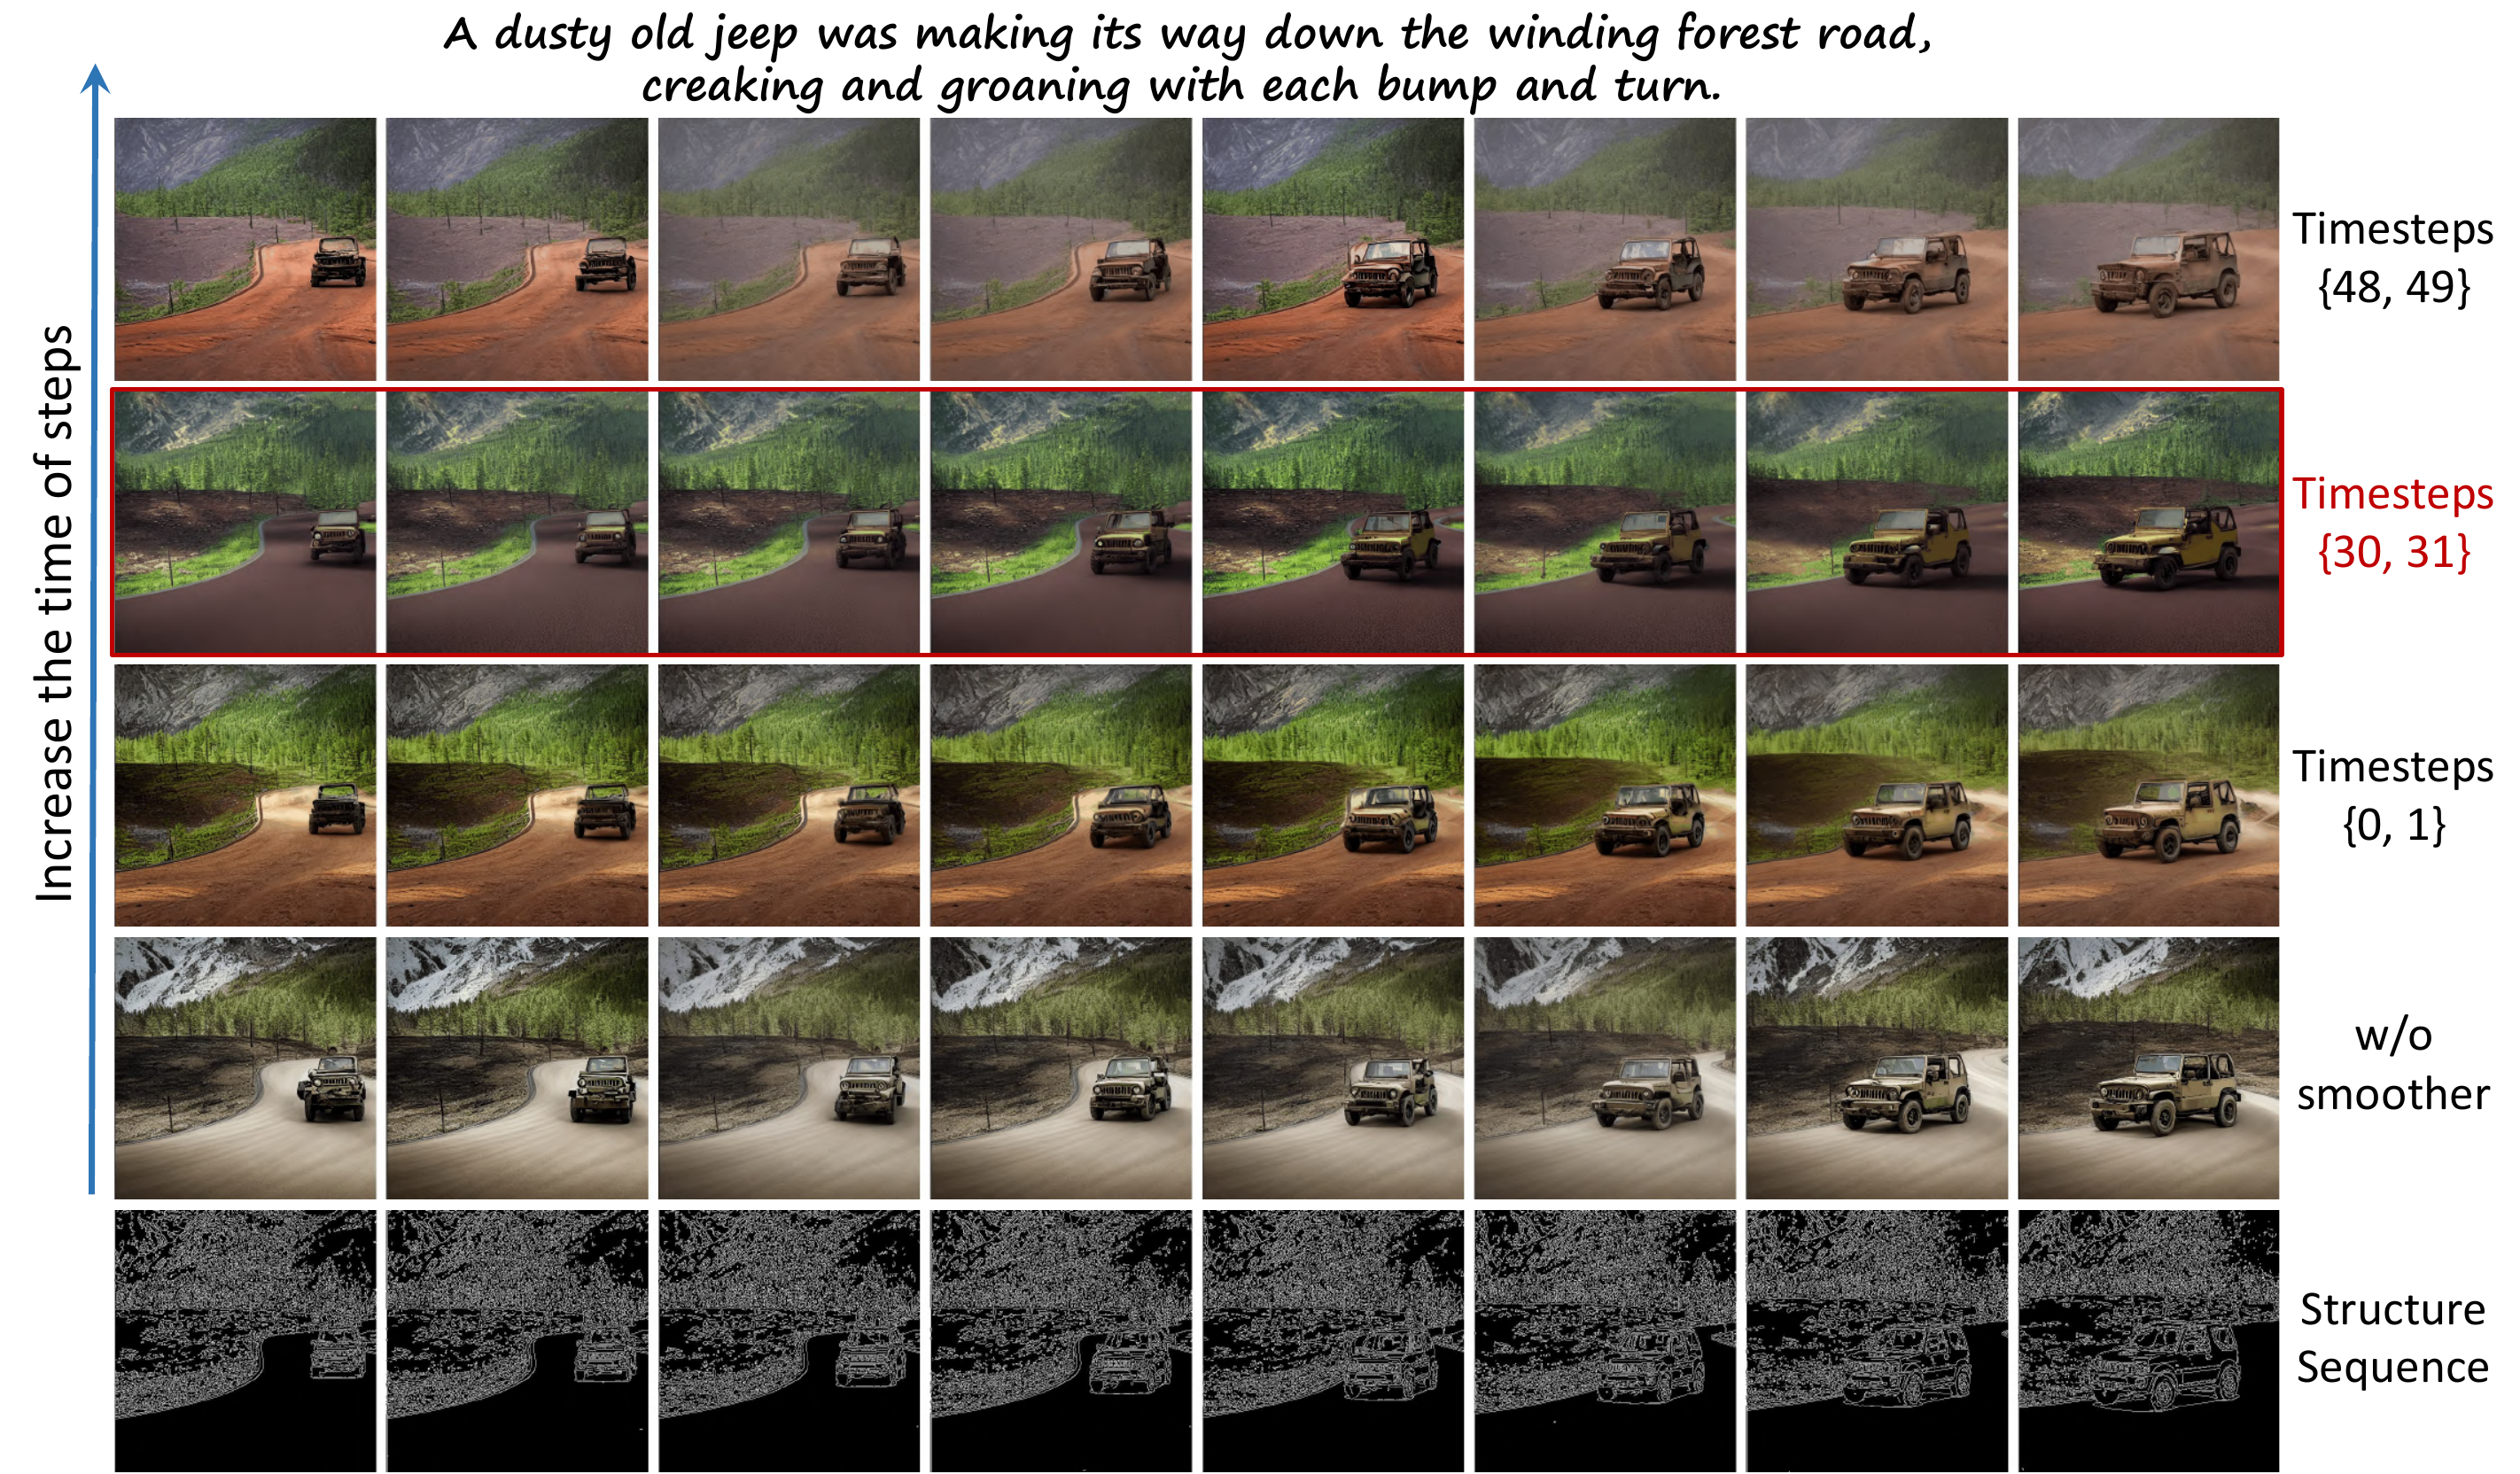}
  \end{center}
  \vspace{-1mm}
  \caption{
  \textbf{.}
  \textbf{Results best seen at 500\% zoom.}
  }
    \label{fig:ab_smoother_time}
  \vspace{-1mm}
\end{figure}

\begin{figure}[t]
%   \vspace{-1em}
  \begin{center}
  \includegraphics[width=.95\linewidth]{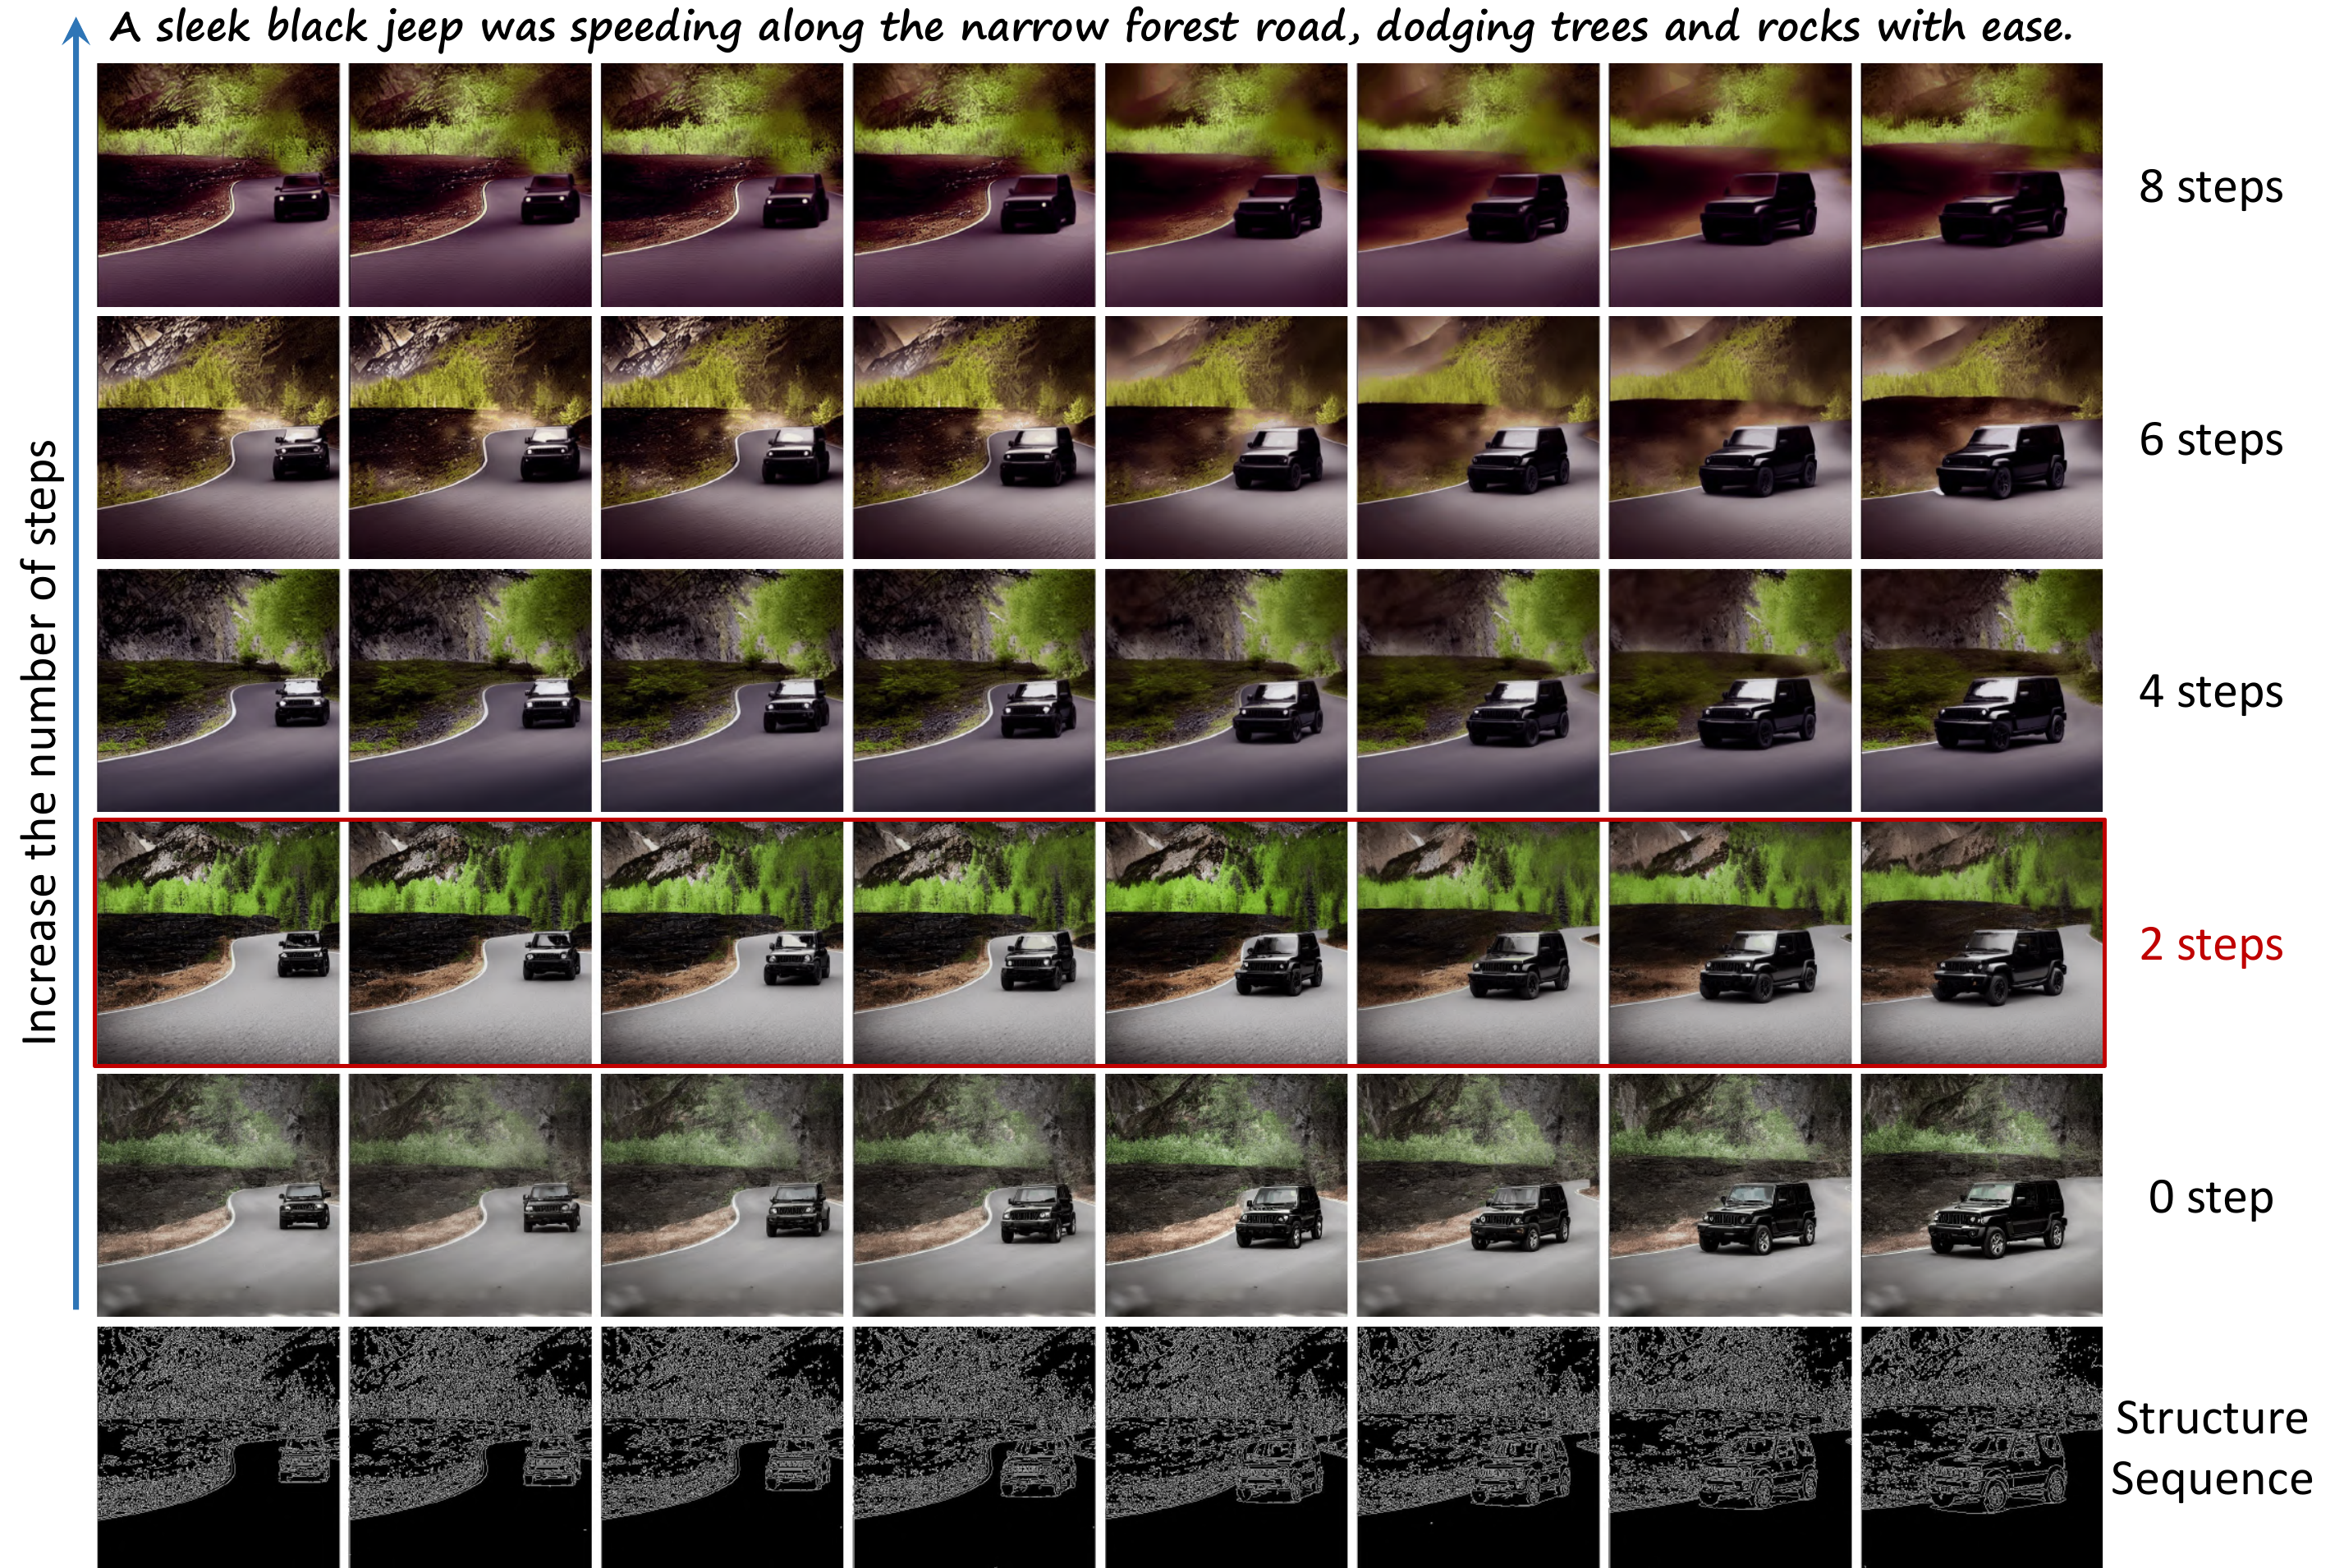}
  \end{center}
  \vspace{-1mm}
  \caption{
  \textbf{.}
  \textbf{Results best seen at 500\% zoom.}
  }
    \label{fig:ab_smoother_number}
  \vspace{-1mm}
\end{figure}
