# Supplementary material for: ControlVideo: Training-free Controllable Text-to-Video Generation
Source: arXiv:2305.13077 source file (2023-05-22)
Supplement: Supplementary file 4 [file supp_data.tex]

\begin{table}[t]
\caption{
    \textbf{Names and captions of selected videos from DAVIS dataset.}}
    \vspace{2mm}
    \centering
    \scalebox{0.9}{
    \begin{tabular}{lc}
    \toprule
         \makecell{Video Name} & \makecell{Source Caption} \\
         % \Xhline{\arrayrulewidth}
         \midrule
         blackswan &{a black swan moving on the lake} \\
         boat &{a boat moves in the river} \\
         breakdance-flare &{a man dances on the road} \\
         bus &{a bus moves on the street} \\
         camel &{a camel walks on the desert} \\
         car-roundabout &{a jeep turns on a road} \\
         car-shadow &{a car moves to a building} \\
         car-turn &{a jeep on a forest road} \\
         cows &{a cow walks on the grass} \\
         dog &{a dog walks on the ground} \\
         elephant &{an elephant walks on the ground} \\
         flamingo &{a flamingo wanders in the water} \\
         gold-fish &{golden fishers swim in the water} \\
         hike &{a man hikes on a mountain} \\
         hockey &{a player is playing hockey on the ground} \\
         kite-surf &{a man is surfing on the sea} \\
         lab-coat &{three women stands on the lawn} \\
         longboard &{a man is playing   skateboard on the alley} \\
         mallard-water &{a mallard swims on the water} \\
         mbike-trick &{a man riding motorbike} \\
         rhino &{a rhino walks on the rocks} \\
         surf &{a sailing boat moves on the sea} \\
         swing &{a girl is playing on the swings} \\
         tennis &{a man is playing tennis} \\
         walking &{a selfie of walking man} \\
    \bottomrule
    \end{tabular}
    }
    % \vspace{-2mm}
    \label{tab:supp_data}
\end{table}
